# Supplementary material for: Terahertz-optical intensity grating for creating high-charge, attosecond electron bunches
Source: arXiv:1808.01737 ancillary file (2019-04-18)
Supplement: Supplementary file 1 [file Supp_info.pdf]

# Terahertz-optical intensity grating for creating high-charge, attosecond electron bunches

Jeremy Lim and Yidong Chong

School of Physical and Mathematical Sciences, Nanyang Technological University

Liang Jie Wong

Singapore Institute of Manufacturing Technology (SIMTech), A*STAR

## Supporting Information

**Contents** **page**

**S.1 Electron dynamics in continuous wave intensity gratings…………………………2**

**S.2 Electron dynamics without longitudinal momentum spread in pulsed intensity gratings……………………………………………………………………………………9**

**S.3 Dynamics of quasi-monoenergetic electrons in pulsed intensity gratings……….20**

**S.4 Limitations of analytical formulation……………………………………………...27**

**S.5 Methods and parameters used in main text**

**S.5 (i) Numerical integration of the equations of motion…………………….30**

**S.5 (ii) Exact, finite-energy, pulsed solutions to Maxwell's equations……….31**

**S.5 (iii) Initial electron phase space distributions……………………………...32**

**S.5 (iv) Case 1 parameters: low-charge, low-KE spread electron bunch…….33**

**S.5 (v) Case 2 parameters: 20 fC, 7 fs, 8 µm-radius electron bunch………...34**

**S.5(vi) Parameters used to plot results in main text Figure 3………………..35**

## S.1 Electron dynamics in continuous wave intensity gratings

In this section, we consider the longitudinal dynamics of electrons interacting with an intensity grating formed by overlapping, counter-propagating, continuous EM plane waves (CW). We operate in the rest frame of the electron (herein also called the primed frame) which moves at velocity $\vec{v} = +\beta_0 c\,\hat{z}$ with respect to the lab frame. As we have shown using equation (1) in the main text, the frequencies of the EM waves can be chosen to match specific mean electron velocities. We show that in the primed frame, electrons near the intensity minima form the high-density bunch core after compression and that they can be treated as simple harmonic oscillators (SHO). This allows us to derive analytical formulae for the period between maximum compression and the associated stiffness constant, $K_0'$, with explicit dependence on peak electric field strengths used and polarization angle. These scaling trends provide us with a crude, albeit helpful, preliminary constraints on parameter selection for the more realistic case where the intensity grating is synthesized from counter-propagating pulsed EM waves.

The corresponding Lorentz factor is $\gamma_0 = 1/\sqrt{1-\beta_0^2}$. We assume the electrons are non-interacting and have no longitudinal momentum spread. We study the regime in which both the initial and grating-induced motion in the primed frame are non-relativistic – valid for electron bunches with small energy spreads typical of UEI beamlines, as we have mentioned in the main text. Considering only primed frame dynamics allows us to refrain from making the distinction between the relativistic and non-relativistic regimes, which would be required if we were to study the problem in the lab frame. First, we derive the form of the ponderomotive force beginning with the primed frame Lorentz force equation:

$$\frac{d\vec{p}'}{dt'} = -e\left(\vec{E}' + \vec{v}' \times \vec{B}'\right). \tag{S1}$$

Primed superscripts denote quantities as observed in the primed frame. Ideally, the longitudinal fields, $E_z'$ and $B_z'$, vanish. Under these assumptions, and using the following expressions (in the Lorenz gauge in source and current-free regions in a vacuum):

$$\vec{E}' = -\frac{\partial \vec{A}'}{\partial t'}, \tag{S2}$$

$$\vec{B}' = \nabla \times \vec{A}', \tag{S3}$$

we can decompose (S1) into transverse (subscript "⊥") and longitudinal terms (in $z'$) solely in terms of the vector potential, $\vec{A}'$:

$$\frac{d\vec{p}'_\perp}{dt'} = e\left(\frac{\partial \vec{A}'}{\partial t'} + v'_z \frac{\partial \vec{A}'}{\partial z'}\right) = \frac{d\vec{A}'}{dt'} \ , \tag{S4}$$

$$\frac{dp'_z}{dt'} = -e\vec{v}' \cdot \left(\frac{\partial \vec{A}'}{\partial z'}\right) . \tag{S5}$$

Straight-forward integration of (S4) with respect to time yields the transverse momenta:

$$\vec{p}'_\perp = e\left(\vec{A}'_\perp + \vec{C}'_\perp\right) , \tag{S6}$$

where $\vec{C}'_\perp = \left(C'_{p_x}, C'_{p_y}\right)$ is the vector containing the constants of integration determined by the initial transverse momenta. Using (S6) and $\vec{p}' = m_e\vec{v}'$, (S5) becomes:

$$\frac{dp'_z}{dt'} = F'_z = -\frac{e^2}{2m_e}\left[\frac{\partial}{\partial z'}\left(\vec{A}' \cdot \vec{A}'\right)\right] + \frac{e^2}{m_e}\left[\frac{\partial}{\partial z'}\left(\vec{A}'_\perp \cdot \vec{C}'_\perp\right)\right] . \tag{S7}$$

Performing time averaging, defined by the operator $\langle f(t')\rangle = \delta t'^{-1}\int_{t'_0}^{t'_0+\delta t'} f(t')dt'$ over the time interval $\delta t'$, we get the ponderomotive force expression, $F'_P$:

$$\langle F'_z\rangle = F'_P = -\frac{e^2}{2m_e}\left\langle \frac{\partial}{\partial z'}\left(\vec{A}' \cdot \vec{A}'\right)\right\rangle + \frac{e^2}{m_e}\left\langle \frac{\partial}{\partial z'}\left(\vec{A}' \cdot \vec{C}'_\perp\right)\right\rangle . \tag{S8}$$

For EM waves, the characteristic time-scale over which time-averaging should be carried out would be a single EM wave period, $T' = \lambda'/c$, where $\lambda'$ is the doppler-shifted EM wavelength. A natural length-scale against which changes in $z'$ can be compared against would be the intensity grating period, $\lambda'_{gr} = \lambda'/2$. We now show that if the primed frame longitudinal dynamics are non-relativistic, on time-scales similar to $T'$, changes in $z'$ will be negligible compared to $\lambda'_{gr}$, and we may treat the partial derivative operator with respect to $z'$ and the time-averaging operator over a single optical cycle as commutating. Consider the small longitudinal primed frame displacement, $\delta z'$, over a time interval $\delta t' = T'$

$$\delta z' = z'(t' + T') - z'(t') = v'_z T'. \tag{S9}$$

We assume the instantaneous velocity, $v'_z$, does not change in the interval $\delta t' = T'$. We now impose the condition that $\delta z'$ should be dwarfed by $\lambda'_{gr}$,:

$$\delta z' = v'_z T' \ll \lambda'_{gr} = \frac{\lambda'}{2} . \tag{S10}$$

Since $\lambda' = T'c$, we get the following inequality:

$$\frac{v_z'}{c} \ll \frac{1}{2} \, , \tag{S11}$$

which is consistent with our assumption that all primed frame dynamics should be non-relativistic. Hence, (S8) can be restated as

$$F_P' = -\frac{\partial}{\partial z'}\left(\frac{e^2}{2m_e}\langle \vec{A}' \cdot \vec{A}' \rangle\right) = -\frac{\partial U_P'}{\partial z'} \, , \tag{S12}$$

where the ponderomotive potential is denoted $U_P'$. The second term in (S8) vanishes when the time-averaging and partial derivative operators are interchanged since $\vec{A}'$ is (co)sinusoidal in $t'$. Since $\vec{A}' \propto \vec{E}'$, this implies that $\vec{A}' \cdot \vec{A}' \propto \left|\vec{E}'\right|^2$. Since the intensity of the fields is proportional to $\left|\vec{E}'\right|^2$, it follows that $\vec{A}' \cdot \vec{A}'$, and thus $U_P'$, is proportional to the intensity. Hence, it can be seen from (S12) that the ponderomotive force pushes electrons (all charged particles in general) longitudinally from higher to lower intensity regions in the frame where motion is non-relativistic.

We now consider a counter-propagating, linearly-polarized (LP) plane wave configuration given by the primed frame vector potential expressions:

$$\vec{A}_1' = \frac{E_{01}'}{\omega'}\begin{bmatrix}\cos\theta_1 \\ \sin\theta_1 \\ 0\end{bmatrix}\sin(k'z' - \omega't' + \phi_{01}') \, , \tag{S13}$$

$$\vec{A}_2' = -\frac{E_{02}'}{\omega'}\begin{bmatrix}\cos\theta_2 \\ \sin\theta_2 \\ 0\end{bmatrix}\sin(k'z' + \omega't' + \phi_{02}') \, . \tag{S14}$$

Subscripts “1” and “2” denote the quantities of the co-propagating and counter-propagating EM waves respectively. The constant phase shifts of each wave are denoted $\phi_{01}'$ and $\phi_{02}'$. When the $z'$ axis is pointing into the page, the angles $+\theta_1$ and $+\theta_2$ are the angles swept out clockwise with respect to the $x$-axis by the electric field polarization vectors. Substituting (S13) and (S14) into the expression for $U_P'$ given by the bracketed term in (S12), we get the form of the spatially-dependent ponderomotive potential:

$$U'_P = \frac{e^2 {E'_{01}}^2}{2m_e \omega'^2}\left[\frac{1}{2}(1+n'^2) + n'\cos(\phi'_{01}+\phi'_{02})\cos\Delta\theta \right.$$
$$\left. - 2n'\cos\Delta\theta \sin(k'z'+\phi'_{01}+\phi'_{02})\sin k'z' \right] . \quad \text{(S15)}$$

The doppler-shifted angular frequency is $\omega' = 2\pi c/\lambda'$ and the corresponding wavenumber is $k' = 2\pi/\lambda'$. The amplitude ratio is $n' = E'_{02}/E'_{01}$ and $\Delta\theta$ is the absolute relative angle separating both polarization vectors. The sine-squared (up to some phase shift $\phi'_{01}+\phi'_{02}$) longitudinal spatial dependence is clear. About the minima of the intensity grating, we may approximate $U'_P$ as a parabolic potential by performing a Taylor's expansion up to second order in $(z'-z'_{min})$, where $z'_{min}$ is the primed frame intensity minima position such that $k'z'_{min} = [(2l+1)\pi - \phi'_{01} - \phi'_{02}]/2$ for $l \in \mathbb{Z}$:

$$U'_P = \frac{1}{2}K'_0(z'-z'_{min})^2 + \cdots . \quad \text{(S16)}$$

The ellipses hide the higher-order terms, which we neglect. $K'_0$ is the stiffness constant which takes the form:

$$K'_0 = \left.\frac{\partial^2 U'_P}{\partial z'^2}\right|_{k'z'_{min}} = \frac{2e^2 E'_{01}E'_{02}\cos\Delta\theta}{m_e c^2} . \quad \text{(S17)}$$

The electrons subjected to this parabolic potential can be treated as SHOs and are subjected to the restoring force $F_P = -K'_0(z'-z'_{min})$. The associated primed frame angular frequency and period of oscillation are $\Omega'_{SHO} = \sqrt{K'_0/m_e}$ and $T'_{SHO} = 2\pi/\Omega'_{SHO}$ respectively. Since the electrons which are subjected to the parabolic potential have $T'_{SHO}$ independent of their initial positions, they cross the intensity minima periodically at the same time, forming a high density region centred at $z_{min}$. These times are defined to be the points of maximum compression. The electrons outside the parabolic potential region have larger oscillation periods dependent on their initial deviation from $z'_{min}$ and do not contribute to the high density bunch core formation. Hence, it suffices to consider only the electrons within the immediate vicinity of $z'_{min}$. These electrons cross the $z_{min}{}'$ twice per oscillatory period, which implies that the primed frame interval between successive maximum compressions is:

$$\Delta T'_{foc} = \frac{T'_{SHO}}{2} = \frac{\pi m_e c}{e\sqrt{2E'_{01}E'_{02}\cos\Delta\theta}} . \quad \text{(S18)}$$

In the lab frame, this time interval is dilated: $\Delta T_{foc} = \gamma_0 \Delta T'_{foc}$, where $\gamma_0 = 1/\sqrt{1-\beta_0^2}$ . It can be observed that polarization vectors which are orthogonal to each other results in (S18) diverging. This simply implies that no compression occurs. This is to be expected since configurations with orthogonal $\vec{E}$-field vectors will have resultant $\vec{E}$ and $\vec{B}$ field vectors which are either parallel or anti-parallel, implying that the $\vec{v} \times \vec{B}$ term, responsible for the ponderomotive force-driven motion, vanishes.

Intensity gratings can also be constructed from circularly polarized (CP) waves. Consider the following vector potential configuration:

$$\vec{A}'_1 = \frac{E'_{01}}{\omega'} \begin{bmatrix} \sin(k'z' - \omega't' + \phi'_{01}) \\ -\cos(k'z' - \omega't' + \phi'_{01}) \\ 0 \end{bmatrix} , \tag{S19}$$

$$\vec{A}'_2 = \frac{E'_{02}}{\omega'} \begin{bmatrix} -\sin(k'z' + \omega't' + \phi'_{02}) \\ -\cos(k'z' + \omega't' + \phi'_{02}) \\ 0 \end{bmatrix} . \tag{S20}$$

Glozing over tedious manipulation, we arrive at the ponderomotive potential expression:

$$\begin{aligned} U'_P = \frac{e^2 {E'_{01}}^2}{2m_e\omega'^2} &\{[1 + n'^2 - 2n' \cos(\phi'_{01} + \phi'_{02})] \\ &+4n' \cos k'z' \cos(k'z' + \phi'_{01} + \phi'_{02})\} . \end{aligned} \tag{S21}$$

The corresponding stiffness constant, $K'_0$ , obtained once again by Taylor's expansion to second order in $(z' - z'_{min})$, takes the form:

$$K'_0 = \frac{4E'_{01}E'_{02}e^2}{m_e c^2} . \tag{S22}$$

The corresponding primed frame interval between successive maximum compressions for the CP configuration is:

$$\Delta T'_{foc} = \frac{\pi m_e c}{2e\sqrt{E'_{01}E'_{02}}} . \tag{S23}$$

We only consider the use of LP EM wave configurations in the main text.

Figure S1 shows our numerical results for 500 initially monoenergetic, non-interacting 31 keV electrons being compressed by an intensity grating formed from counter-propagating, CW LP plane EM waves. The simulations were carried out in the lab frame and the plots were obtained by performing a Lorentz transform into the primed frame, in which they occupy one

ponderomotive grating period $\lambda'_{grating} = \pi/k'$. The figure caption lists the parameters used. The primed frame time interval between successive compressions is predicted by (S18) to be $\Delta T'_{foc} \sim 535$ fs. We use the inverse participation ratio (IPR) quantity to identify areas of high localization (and thus compression). For each time step $t'_j$ the IPR is given by [1]:

$$\mathrm{IPR}(t'_j) = \frac{\sum_{i=1}^{N}\left[\rho_i(t'_j)^2\right]}{\left[\sum_{i=1}^{N}\rho_i(t'_j)\right]^2} \ . \qquad \text{(S24)}$$

For each state $i$ corresponding to spatial width $\Delta z'_i$ such that $N\Delta z'_i = \lambda'_{grating}$, the probability density of finding an electron in $\Delta z'_i$ at time $t'_j$ is $\rho(t'_j)$. Probability density in this context merely refers to the fraction of all electrons which can be found in each differential element $\Delta z'_i$. A large IPR value indicates that a large fraction of electrons are distributed across a small number of states while a small IPR values indicate that all electrons are almost evenly distributed across the potential well. Hence, IPR is a useful tool in identifying the times at which the spatial distribution is sharply peaked, which occurs when most of the electrons are localized at the intensity minimum, and the bunch is maximally compressed.

With reference to Figures. S1(a)-(c), the IPR peaks coincide almost exactly with the predicted times of compression given by Eq. (S18). However, the discrepancy between them increases with each subsequent compression. This stems from our use of the parabolic potential to model the region about the minima. The vast majority of electrons lie outside the region where this potential is valid. Thus, their oscillation period increases with their deviation from the intensity minima. Even if these deviations are minute, the slight delays in crossing the intensity minima are compounded over time, leading to IPR peaks which become increasingly delayed with respect to the predicted times – which is what is observed. The IPR peak values for each subsequent compression also decreases. This is due to the increase in number of localization regions, also attributed to the deviation of the actual potential from the intensity minimum. This is evident from Figures. S1(d)-(f), where the two additional regions of higher localization appear with each subsequent compression. Hence, the highest density peak is attained at the first compression. This means that the pulse durations chosen for the pulsed-laser case should result in attosecond-long bunches formed during the first compression. As a preliminary constraint, this implies that the pulse overlap time should be less than $\Delta T'_{foc}$.

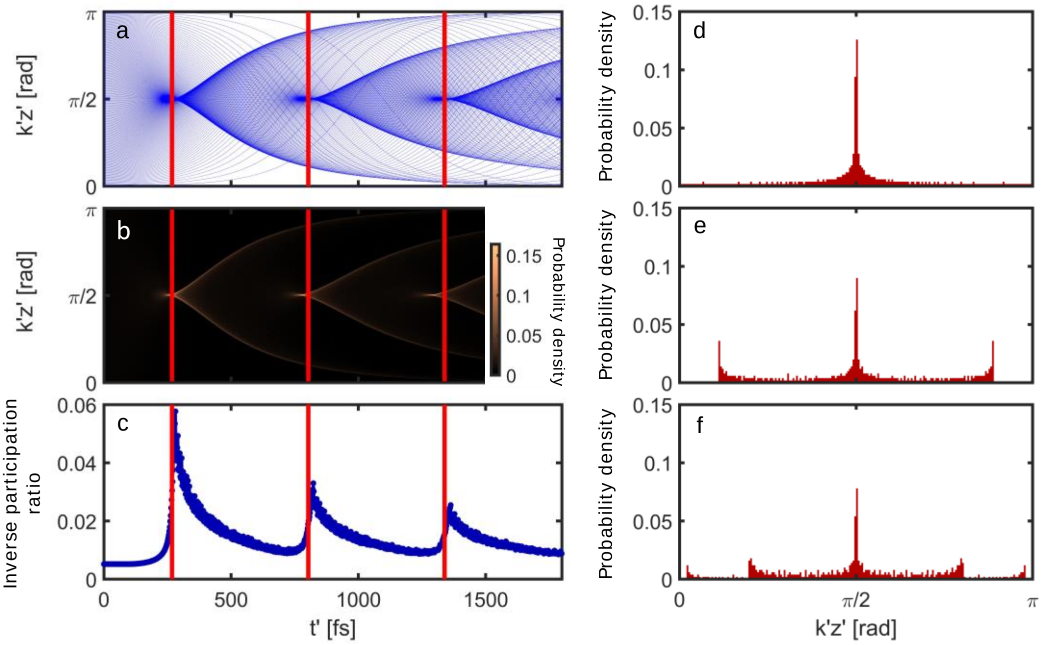


**Figure S1: Primed frame, single ponderomotive well dynamics of 500 non-interacting, mono-energetic electrons in an linearly-polarized (LP), continuous EM plane wave (CW) intensity grating.** The electron kinetic energy was 31 keV, which is matched by wavelengths $\lambda_1 = 0.4\ \mu$m and $\lambda_2 = 2\lambda_1$. The field strengths used were $E_{01} = 10^{10}$ V/m and $E_{02} = E_{01}/2$. We chose $\Delta\theta = 0$ for simplicity. (a) The solid blue lines are the numerically-computed lab-frame longitudinal electron trajectories, $z'(t')$, after performing a Lorentz transform into the electron rest frame. The corresponding electron density heat map evolution in $t'$ is plotted in (b). The brighter areas indicate regions of high electron density. (c) shows a plot of the corresponding inverse participation ratio (IPR), given by (S24). A higher IPR value indicates greater localization, indicating compression. The vertical solid red lines plotted in (a), (b), and (c) are the predicted times of compression given by (S18), which are in close agreement with the times of high localization. (d)-(f) depict the probability distribution of electrons within the potential well at the first, second, and third predicted times of compression respectively.

Figure S2 depicts a comparison between the analytically predicted scaling of the time to first compression as a function of amplitude ratio and relative polarization angle, shown in panels (a) and (b) respectively. We chose to consider only the time to the first compression as we have previously determined that it results in the most sharply-peaked spatial distribution. It can be seen from figure S2 that our expectations are in perfect agreement with the numerics for both the LP and CP cases.

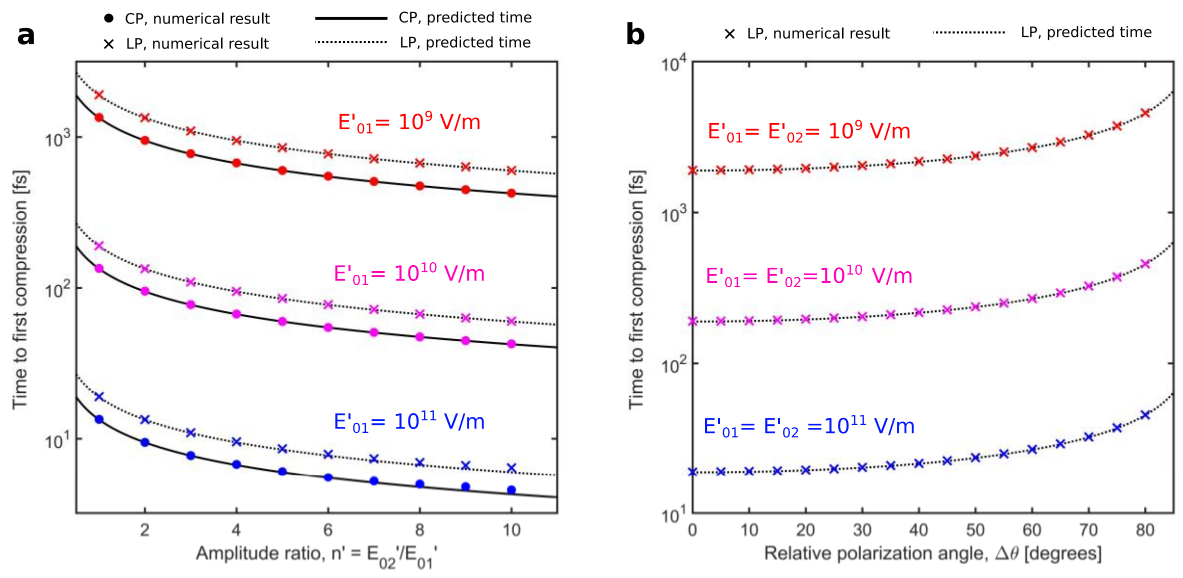


**Figure S2: Dependence of primed frame compression times on EM wave amplitudes, polarization configuration (CP and LP), and relative angle of polarization for the LP case.** (a) shows both the analytical and numerical scaling trend of the prime frame time to first compression as a function of the amplitude ratio $n' = E'_{02}/E'_{01}$ for both the LP and CP cases. (b) shows the time to first compression as a function of relative polarization angle, $\Delta\theta$ for the LP case. The predicted time to first compression is defined to be $\Delta T'_{foc}/2$. The data points denote the numerically obtained results and the lines denote the analytical prediction given by (S18) for the LP case, and (S23) for the CP case.

In summary, we have derived an expression for the primed frame time interval between maximum compressions by invoking the SHO approximation for the CP and LP cases. We have shown that our expectations agree exactly with the numerical results and that the first compression provides the highest quality attosecond electron bunch, providing us with a preliminary constraint for the pulse durations which should be used for the pulsed EM wave case.

## S.2 Electron dynamics without longitudinal momentum spread in pulsed intensity gratings

In this section, we consider a non-interacting electron bunch, with no longitudinal momentum spread, compressed by an intensity grating formed from overlapping, counter-propagating, pulsed EM plane waves. We derive a closed-form expression for the primed frame time between interaction and maximum compression (focal time) using a perturbative approach and show that it is in good agreement with single-electron numerical simulations in the pulsed EM plane wave limit.

We consider longitudinal electron dynamics within plane waves modulated by Gaussian profiles and vanishing longitudinal fields. We substitute a zeroth-order trajectory solution ${z'}^{(0)}(t') = \beta'_{z,i}ct' + z'_0$ into the Lorentz force equation and solve for the first-order trajectory and velocity expressions ${z'}^{(1)}(t')$ and ${\dot{z}'}^{(1)}(t')$ respectively. The initial ($t' = t'_0 =$ 0 s) primed frame electron position and velocity are denoted $z'_0$ and $\beta'_{z,i}c$ respectively. Setting $\beta'_{z,i} = 0, {z'}^{(0)}(t') = z'_0$ corresponds to a stationary-particle trajectory. We once again consider only the regime in which both the initial and grating-induced motion in the primed frame are non-relativistic: $\beta' = \sqrt{{\beta'_x}^2 + {\beta'_y}^2 + {\beta'_z}^2} \ll 1$, and $\beta'_x, \beta'_y, \beta'_z \ll 1$. We have denoted $\beta'_x = \dot{x}'/c$, $\beta'_y = \dot{y}'/c$, and $\beta'_z = \dot{z}'/c$, with the overdots representing the total derivative with respect to $t'$.The primed frame Lorentz factor is $\gamma' = 1/\sqrt{1 - {\beta'}^2} \approx 1$. Accordingly, our first-order equations of motion reduce to:

$$\ddot{x}'^{(1)}(t') = -\frac{e}{m_e}\left(E'_x - \beta'_{z,i}cB'_y\right), \tag{S25}$$

$$\ddot{y}'^{(1)}(t') = -\frac{e}{m_e}\left(E'_y + \beta'_{z,i}cB'_x\right), \tag{S26}$$

$$\ddot{z}'^{(1)}(t') = -\frac{e}{m_e}\left(\dot{x}'^{(1)}B'_y - \dot{y}'^{(1)}B'_x\right) . \tag{S27}$$

We consider counter-propagating LP EM plane waves modulated by a Gaussian pulse shape. For the co-propagating wave, the fields are:

$$\vec{E}'_1 = E'_{01}\mathcal{G}'_1 \begin{bmatrix} \cos\theta_1 \\ \sin\theta_1 \\ 0 \end{bmatrix} \cos\eta'_1 , \tag{S28}$$

$$\vec{B}'_1 = \frac{E'_{01}}{c}\mathcal{G}'_1 \begin{bmatrix} -\sin\theta_1 \\ \cos\theta_1 \\ 0 \end{bmatrix} \cos\eta'_1 . \tag{S29}$$

For the counter-propagating waves, the fields are:

$$\vec{E}'_2 = n'E'_{01}\mathcal{G}'_2 \begin{bmatrix} \cos\theta_2 \\ \sin\theta_2 \\ 0 \end{bmatrix} \cos\eta'_2 , \tag{S30}$$

$$\vec{B}'_2 = \frac{n'E'_{01}}{c}\mathcal{G}'_2 \begin{bmatrix} \sin\theta_2 \\ -\cos\theta_2 \\ 0 \end{bmatrix} \cos\eta'_2 . \tag{S31}$$

We have defined $\theta_1$, $\theta_2$, and $n'$ in section S.1. Once again, subscripts "1" and "2" denote co-propagating and counter-propagating wave quantities respectively. The wave phases are denoted:

$$\eta_1' = k'z_0' - \omega' t' + \phi_{01}' \,, \tag{S32}$$

$$\eta_2' = k'z_0' + \omega' t' + \phi_{02}' \,. \tag{S33}$$

The modulating Gaussian envelopes are:

$$\mathcal{G}_1'(t') = \exp\left[-\frac{1}{T_1'^2}\left(\frac{z_0' - z_{i,1}'}{c} - t'\right)^2\right] , \tag{S34}$$

$$\mathcal{G}_2'(t') = \exp\left[-\frac{1}{T_2'^2}\left(\frac{z_0' - z_{i,2}'}{c} + t'\right)^2\right] . \tag{S35}$$

The primed frame Gaussian pulse durations are $T_1'$ and $T_2'$. The initial position of the pulse peaks along the $z'$-axis at are $z_{i,1}'$ and $z_{i,2}'$. We assume the Gaussians vanish at the initial time, implying that there are no fields in the region of interaction initially. We use the following approximation when integrating the equations of motion:

$$\int \mathcal{G}' \cos \eta' dt' \approx \mathcal{G} \int \cos \eta' dt', \tag{S36}$$

where the $\cos \eta'$ term can be replaced with $\sin \eta'$ as well. This approximation is valid for the integral evaluated at times long before and after the electron-grating interaction (i.e. where and when the Gaussian terms vanish), which, as we shall subsequently show, are the times of interest.

Substituting the zeroth-order solution $z'^{(0)}(t') = z_0'$ into the transverse force components, (S25) and (S26), setting $\beta_{z,i}' = 0$ , and invoking approximation (S36) when integrating with respect to $t'$, we get the transverse first-order velocities:

$$\dot{x}'^{(1)}(t') \approx \frac{eE_{01}'}{m_e \omega'}\left(\mathcal{G}_1' \cos\theta_1 \sin\eta_1' - n'\mathcal{G}_2' \cos\theta_2 \sin\eta_2' + C_{v_x}'\right), \tag{S37}$$

and

$$\dot{y}'^{(1)}(t') \approx \frac{eE_{01}'}{m_e \omega'}\left(\mathcal{G}_1' \sin\theta_1 \;\sin\eta_1' - n'\mathcal{G}_2' \sin\theta_2 \;\sin\eta_2' + C_{v_y}'\right), \tag{S38}$$

where $C'_{v_x}$ and $C'_{v_y}$ are the constants of integration which depend on the initial transverse velocities, $\dot{x}'_0$ and $\dot{y}'_0$, which are given by:

$$C'_{v_x} = \frac{m_e \omega'}{eE'_{01}} \dot{x}'_0 \tag{S39}$$

and

$$C'_{v_y} = \frac{m_e \omega'}{eE'_{01}} \dot{y}'_0 \,. \tag{S40}$$

Since only the longitudinal trajectories are of interest, we do not solve for the transverse ones. We substitute (S37) and (S38) into (S27) and integrate with respect to time, once again invoking approximation (S36), yielding the primed frame longitudinal velocity:

$$\begin{aligned} \dot{z}'^{(1)}(t') \approx -\frac{e^2 {E'_{01}}^2}{m_e^2 c} \Bigg\{ & \frac{1}{4\omega'^2} {\mathcal{G}'_1}^2 \cos 2\eta'_1 - \frac{n'^2}{4\omega'^2} {\mathcal{G}'_2}^2 \cos 2\eta'_2 \\ & - \frac{1}{\omega'^2} \mathcal{G}'_1 \left( C'_{v_x} \cos\theta_1 + C'_{v_y} \sin\theta_1 \right) \sin\eta'_1 \\ & - \frac{n'}{\omega'^2} \mathcal{G}'_2 \left( C'_{v_x} \cos\theta_2 + C'_{v_y} \sin\theta_2 \right) \sin\eta'_2 \\ & - \Bigg[ \frac{n' T'_1}{2\omega'} \sqrt{\frac{\pi}{\alpha_a}} \cos\Delta\theta \sin(2k' z'_0 + \phi'_{01} + \phi'_{02}) \\ & \times \exp\left( \frac{\alpha_b^2 - 4\alpha_a \alpha_c}{4\alpha_a {T'_1}^2} \right) \mathrm{Erf}\left( \frac{2\alpha_a t' + \alpha_b}{2T'_1 \sqrt{\alpha_a}} \right) \Bigg] + C'_{v_z} \Bigg\} . \end{aligned} \tag{S41}$$

The constant of integration $C'_{v_z}$ corresponding to the initial condition $\dot{z}'(t'_0) = 0$ is:

$$C'_{v_z} = -\frac{n' T'_1}{2\omega'} \sqrt{\frac{\pi}{\alpha_a}} \cos\Delta\theta \sin(2k' z'_0 + \phi'_{01} + \phi'_{02}) \exp\left( \frac{\alpha_b^2 - 4\alpha_a \alpha_c}{4\alpha_a {T'_1}^2} \right). \tag{S42}$$

The time-independent constants $\alpha_a$, $\alpha_b$, and $\alpha_c$ are defined such that they satisfy the expression:

$$\mathcal{G}'_1 \mathcal{G}'_2 = \exp\left[ -\frac{1}{T_1'^2} (\alpha_a t'^2 + \alpha_b t' + \alpha_c) \right]. \tag{S43}$$

They have the following forms:

$$\alpha_a = 1 + \frac{T_1'^2}{T_2'^2} \,, \tag{S44}$$

$$\alpha_b = \frac{2}{c}\left[\frac{T_1'^2}{T_2'^2}\left(z_0' - z_{i,2}'\right) - \left(z_0' - z_{i,1}'\right)\right] , \tag{S45}$$

$$\alpha_c = \frac{1}{c^2}\left[\left(z_0' - z_{i,1}'\right)^2 + \frac{T_1'^2}{T_2'^2}\left(z_0' - z_{i,2}'\right)^2\right] . \tag{S46}$$

The error function arises out of the indefinite integral $\int \mathcal{G}_1'\mathcal{G}_2' dt'$ and hints at asymptotic solutions, which suffice in describing the resultant dynamics long after interaction. Integrating (S41) with respect to $t'$ once more yields the first-order primed frame longitudinal trajectory:

$$\begin{aligned} z'^{(1)}(t') \approx -\frac{e^2 E_{01}'^2}{m_e^2 c}\Bigg\{ & -\frac{1}{8\omega'^3}\mathcal{G}_1'^2 \sin 2\eta_1' - \frac{n'^2}{8\omega'^3}\mathcal{G}_2'^2 \sin 2\eta_2' \\ & - \frac{1}{\omega'^3}\mathcal{G}_1'\left(C_{v_x}' \cos\theta_1 + C_{v_y}' \sin\theta_1\right)\cos\eta_1' \\ & + \frac{n'}{\omega'^3}\mathcal{G}_2'\left(C_{v_x} \cos\theta_2 + C_{v_y}' \sin\theta_2\right)\cos\eta_2' \\ & - \frac{n'T_1'}{2\omega'}\sqrt{\frac{\pi}{\alpha_a}}\cos\Delta\theta \exp\left(\frac{\alpha_b^2 - 4\alpha_a\alpha_c}{4\alpha_a T_1'^2}\right)\sin(2k'z_0' + \phi_{01}' + \phi_{02}') \\ & \times\left[\frac{T_1'}{\sqrt{\pi\alpha_a}}\exp\left(-\frac{(2\alpha_a t' + \alpha_b)^2}{4\alpha_a T_1'^2}\right) + \left(\frac{\alpha_b}{2\alpha_a} + t'\right)\mathrm{Erf}\left(\frac{2\alpha_a t' + \alpha_b}{2\sqrt{\alpha_a}T_1'}\right)\right] \\ & + C_{v_z}' t' + C_z' \Bigg\} . \end{aligned} \tag{S47}$$

The constant of integration corresponding to the initial condition $z'(t_0') = z_0'$ is:

$$\begin{aligned} C_z' = -\left\{\frac{\alpha_b}{2\alpha_a}\frac{n'T_1'}{2\omega'}\sqrt{\frac{\pi}{\alpha_a}}\cos\Delta\theta \exp\left(\frac{\alpha_b^2 - 4\alpha_a\alpha_c}{4\alpha_a T_1'^2}\right)\sin(2k'z_0' + \phi_{01}' + \phi_{02}')\right\} \\ - \frac{m_e^2 c}{e^2 E_{01}'^2} z_0' . \end{aligned} \tag{S48}$$

(S41) and (S47) are not necessarily accurate during the time of interaction. From the error function, we can derive an expression for the "centre" of interaction, $t' = t_{center}'$. This can be done by setting the argument of the error function in (S47) to be equal to 0:

$$\mathrm{Erf}\left(\frac{2\alpha_a t'_{center} + \alpha_b}{2T'_1\sqrt{\alpha_a}}\right) = 0 \;\Leftrightarrow\; 2\alpha_a t'_{center} + \alpha_b = 0\,. \tag{S49}$$

Expanding $\alpha_a$ and $\alpha_b$ in full using (S44) and (S45), and substituting $z'_{i,1} = z'_{OL} - ct'_{OL}$ and $z'_{i,2} = z'_{OL} + ct'_{OL}$, we get

$$ct'_{center} = ct'_{OL} + (z'_0 - z'_{OL})\frac{T'^2_2 - T'^2_1}{T'^2_1 + T'^2_2}\,. \tag{S50}$$

We have defined $z'_{OL}$ and $t'_{OL}$ to be the primed frame time and position at which the pulse peaks overlap respectively. The closed form, perturbative first-order solutions to the longitudinal trajectory and velocity are cumbersome and elucidate little information on compression dynamics. However, if we assume that maximum compression of the bunch occurs long after the intensity grating has already faded (no fields), then it suffices for us to study the trajectory in the asymptotic limit $t' \gg t'_{center}$. Evaluating (S41) and (S47) in this limit yields the asymptotic longitudinal trajectory and velocity ($z'_f(t')$ and $\beta'_{z,f} = \dot{z}'_f/c$ respectively):

$$\beta'_{z,f} = \frac{\dot{z}'_f}{c} = \frac{\dot{z}'^{(1)}(t' \gg t'_{center})}{c} = 2\Lambda\frac{e^2 {E'_{01}}^2}{m_e^2 c^2}\sin(2k'z'_0 + \phi'_{01} + \phi'_{02})\ , \tag{S51}$$

$$z'_f(t') = z'^{(1)}(t' \gg t'_{center}) = \beta'_{z,f}ct' + z'_0 + \Lambda\frac{e^2 E'^2_{01}}{m_e^2 c}\frac{\alpha_b}{\alpha_a}\sin(2k'z'_0 + \phi'_{01} + \phi'_{02})\ , \tag{S52}$$

where we have defined the parameter $\Lambda$ to be:

$$\Lambda = \frac{n'\sqrt{\pi}}{2\omega'}\frac{T'_1 T'_2}{\sqrt{T'^2_1 + T'^2_2}}\cos\Delta\theta\,\exp\left[-\frac{4(z'_0 - z'_{OL})^2}{c^2(T'^2_1 + T'^2_2)}\right]. \tag{S53}$$

We have assumed that maximum compression occurs long after interaction which allowed us to set all Gaussian terms to 0 when taking the limit $t' \gg t'_{center}$. By performing ray-tracing and finding the intersection point between the (S52) and $z' = z'_0$, we obtain the time at which all impulse appears to have effectively been imparted. The expression turns out to be exactly the same as (S50), which implies that the centre of interaction time, $t'_{center}$, is also the time when all momentum appears to have been instantaneously imparted. This temporal plane of interaction is akin to the concept of the principal plane in paraxial ray optics, which is the plane of a lens at which all refraction appears to have occurred. Similarly, the principal plane in classical optics can also be obtained by way of ray-tracing.

As we have shown in section S.1 (CW limit), only the electrons close to the intensity minima contribute to the formation of the high density bunch core. As such, we consider only these electrons in the pulsed case. In the temporal lens analogy [2], this is equivalent to the "paraxial" regime where all rays coming from infinity focus onto a single point along the propagation axis. For an intensity grating which goes as $\cos(2k'z_0' + \phi_{01}' + \phi_{02}')$, the minima occur at $k'z_{min}' = [(2l+1)\pi - \phi_{01}' - \phi_{02}']/2, \forall\, l \in \mathbb{Z}$. Thus we expand the $\sin(2k'z_0' + \phi_{01}' + \phi_{02}')$ term in (S51) about these points up to first order with respect to the deviation from the minima, $\Delta z_0'' = z_0' - z_{min}'$. This yields:

$$\dot{z}_f' \approx 2\Lambda|_{k'z_{min}'} \frac{e^2 {E_{01}'}^2}{m_e^2 c} (2k'\Delta z_0''). \tag{S54}$$

Taking maximum compression to be exactly centered at $z_{min}'$ at the time of focus, $t_{foc}'$, the effective time between interaction and focus is:

$$\begin{aligned} t_{foc}' - t_{center}'|_{k'z_{min}'} &= \frac{\Delta z_0''}{2\Lambda|_{k'z_{min}'} \frac{e^2 {E_{01}'}^2}{m_e^2 c}(2k'\Delta z_0'')} \\ &= \frac{m_e}{K_0'\sqrt{\pi}} \sqrt{\frac{1}{T_1'^2} + \frac{1}{T_2'^2}} \exp\left[\frac{4(z_{min}' - z_{OL}')^2}{c^2(T_1'^2 + T_2'^2)}\right], \end{aligned} \tag{S55}$$

where $t_{center}'$ is once again given by Eq. (S50) and $K_0'$ is the stiffness constant in the CW limit given by (S17). While the definition of focal time was defined to be the time between interaction and focus, $t_{center}'$ has dependence on the laser pulse parameters as well as the initial electron positions. In order to shift all parameter dependencies to the RHS of (S55), we modify our definition of focal time, $\Delta t_{foc}'$, slightly:

$$\begin{aligned} \Delta t_{foc}' &= t_{foc}' - t_{OL}' \\ &= \frac{m_e}{K_0'\sqrt{\pi}} \sqrt{\frac{1}{T_1'^2} + \frac{1}{T_2'^2}} \exp\left[\frac{4(z_{min}' - z_{OL}')^2}{c^2(T_1'^2 + T_2'^2)}\right] + \frac{z_{min}' - z_{OL}'}{c} \frac{T_2'^2 - T_1'^2}{T_1'^2 + T_2'^2}. \end{aligned} \tag{S56}$$

Defining the lab frame focal distance to be the spatial separation between the location of focus, $z_{foc} = \gamma_0(z_{foc}' + \beta_0 c t_{foc}')$, and the position where the pulse peaks overlap, $z_{OL} = \gamma_0'(z_{OL}' + \beta_0 c t_{OL}')$, we obtain the expression:

$$f_z = z_{foc} - z_{OL} = \gamma_0\beta_0 c \Delta t_{foc}' + \gamma_0\left(z_{foc}' - z_{OL}'\right)_{z_{foc}' = z_{min}'}. \tag{S57}$$

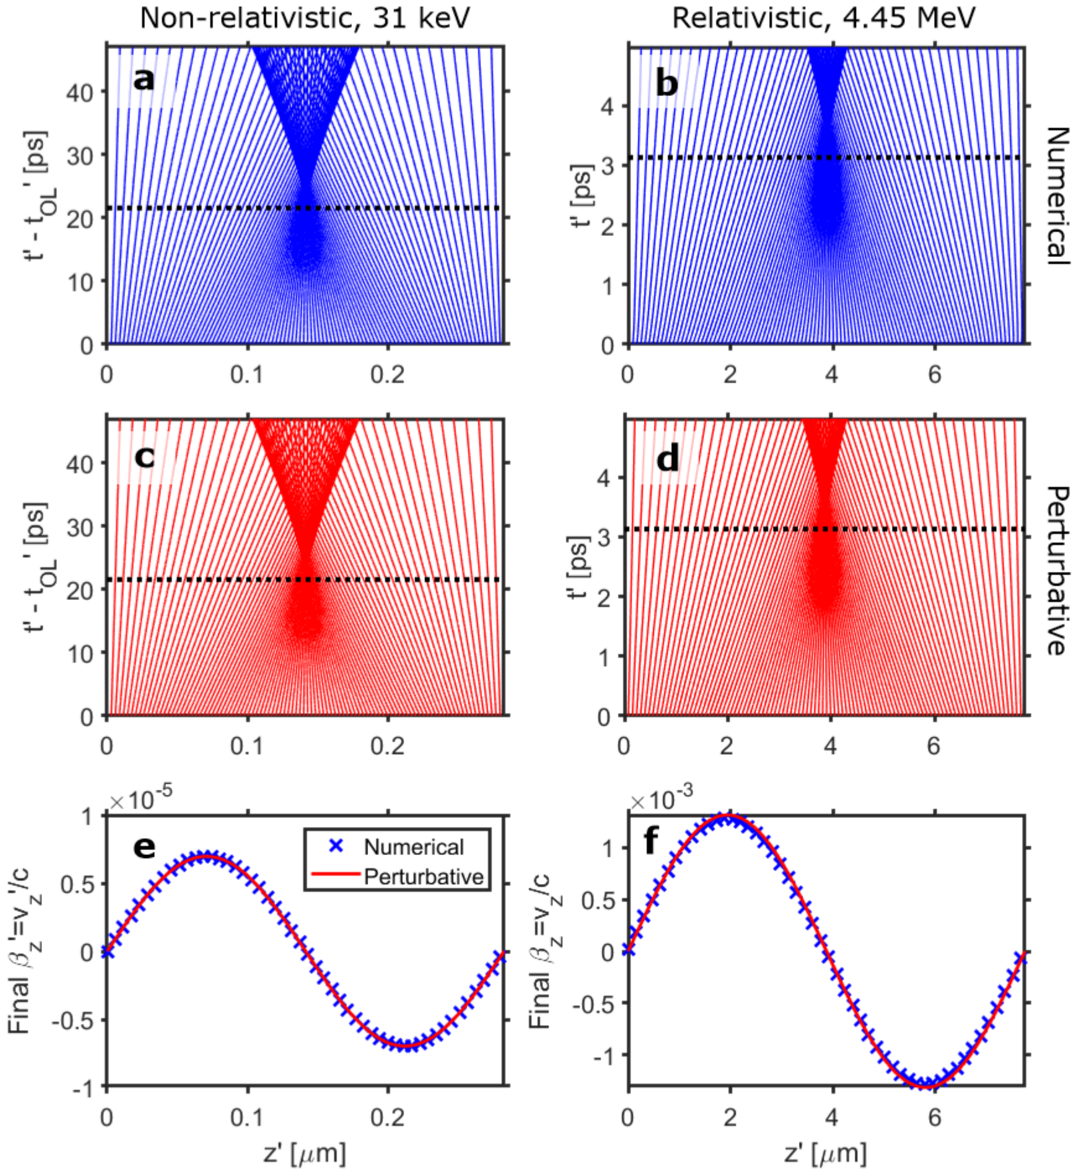


**Figure S3: Comparison between numerically computed trajectories and closed-form, analytical first-order trajectories of electrons being compressed by a pulsed intensity grating in the plane wave limit.** The panels on the left column show the results for a non-relativistic, monoenergetic electron bunch of 31 keV, while those on the right show the results of relativistic, 4.45 MeV monoenergetic electrons. The black dotted lines in (a)-(d) denote the predicted time of focus calculated using Eq. (S56). All simulations were carried out in the lab frame and the resulting trajectories were Lorentz transformed into the primed frame. Table S1 show the parameters used to produce these plots.

Figure S3 compares our analytical trajectories, given by Eq. (S47), with those obtained numerically. Our simulations were carried out in the lab frame with monoenergetic, non-interacting electrons initialized on-axis with uniform separation. We take $\Delta\theta = 0$ here and in the main text for simplicity. The fields used were LP EM plane waves modulated by a Poisson spectrum [3], which is valid in single-cycle limit, tends towards a Gaussian spectrum in the

multi-cycle limit, and does not include unphysical negative frequencies. It can be seen that the closed form primed trajectories are in good agreement with those computed numerically in the lab frame and plotted in the primed frame. The simulation parameters used are listed in table S1.

**Table S1:** List of lab and primed frame parameters used to produce figure S3. Subscripts "1" and "2" denote quantities corresponding to the co-propagating and counter-propagating waves respectively.

| | Parameters | Units | Fig. S3(a) | Fig. S3(c) |
|---|---|---|---|---|
| Lab frame | $E_K$ | eV | $31 \times 10^3$ | $4.45 \times 10^6$ |
| | $\lambda_1$ | $\mu$m | 0.4 | 0.8 |
| | $\lambda_2$ | $\mu$m | 0.8 | 300 |
| | $E_{01}$ | V/m | $1 \times 10^9$ | $1 \times 10^{11}$ |
| | $E_{02}$ | V/m | $0.5 \times 10^9$ | $6 \times 10^7$ |
| | $T_1$ | fs | 76.0 | 25.5 |
| | $T_2$ | fs | 152.0 | 849.3 |
| Primed frame | $E'_{01}$ | V/m | $7.07 \times 10^8$ | $5.16 \times 10^9$ |
| | $E'_{02}$ | V/m | $7.07 \times 10^8$ | $1.16 \times 10^9$ |
| | $T'_1$ | fs | 107.5 | 493.4 |
| | $T'_2$ | fs | 107.5 | 43.9 |

Figure S4 shows a comparison between the predicted and numerically-obtained values of $\Delta t'_{foc}$ as a function of laser pulse amplitude ratio, $n' = E'_{02}/E'_{01}$, and intensity FWHM duration ratio, $n'_T = \tau_{fwhm,1}/\tau_{fwhm,2}$, where $T' = \tau'_{fwhm}/\sqrt{2\log 2}$. The analytical predictions were plotted using Eq. (S56) for various values of durations and amplitudes for the central well, where the middle of the well coincides with $z'_{OL}$. The electrons were initially monoenergetic and initialized on-axis with uniform separation. This time, however, the simulations were carried out in the primed frame since the dynamics in this frame, for a given set of primed frame parameters, are not unique to any specific lab frame kinetic energy value. Our predictions can be seen to be in excellent agreement with our numerical simulations. However, there is a regime in which a large discrepancy arises. This can be observed in the bottom-right region of figure S4(a). The exact $\Delta t'_{foc}$ values no longer follow the trend described by Eq. (S56). This can be attributed to the strong forces exerted by the high field strengths and long pulse durations. As such, compression occurs very close to $t'_{OL}$ and the assumption that

compression occurs long after interaction breaks down. Thus, the electron trajectories do not obey those of free particles at the time of compression, which was a key assumption in deriving Eq. (S56).

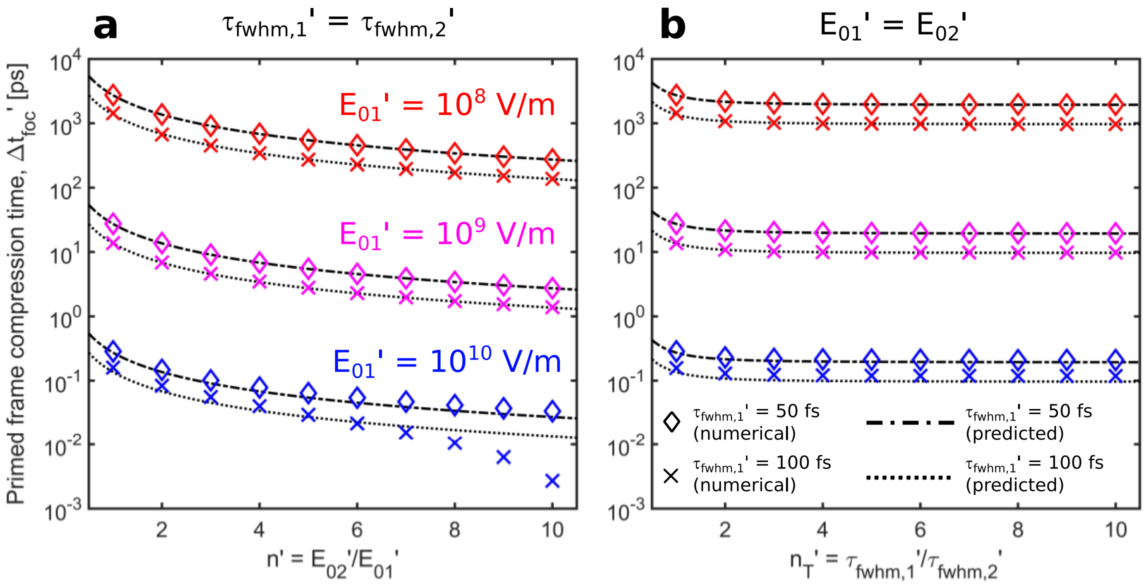


**Figure S4: Dependence of the primed frame time to focus, $\Delta t'_{foc}$, on laser pulse parameters.** The predicted and analytical scaling of the primed frame focal time for monoenergetic electrons are plotted against $n' = E'_{02}/E'_{01}$ for constant intensity FWHM pulse durations, $\tau'_{fwhm}$ in (a), and against $n'_T = \tau'_{fwhm,1}/\tau'_{fwhm,2}$ at constant field amplitude values in (b). The data points and lines represent the numerical and analytical data respectively. The colour of the data markers represent the amplitudes used (labelled) while the type of marker (diamonds or crosses) and line (dashed-dotted or dotted) represent different FWHM durations used. All data except for those in the lower-right area of plot (a) are in excellent agreement with the numerics. The large discrepancy in the aforementioned region arises due to a breakdown in the assumption that compression occurs long after interaction.

In contrast to the work done by Hilbert *et al.* [2], our formulation also accounts for variation in compression behaviour from one potential well to another. The inclusion of the Gaussian envelopes yield such phenomena which are emergent only on length-scales greater than a single grating period, $\lambda_{grating}$. The electron density maps in figure S5 depict the primed frame, time-evolution of the electron density for 7 ponderomotive potential wells. The 4.45 MeV, monoenergetic electrons were initialized on-axis in the lab frame with uniform separation. The electrons are velocity-matched by EM waves of $\lambda_1 = 0.8\,\mu$m and $\lambda_2 = 300\,\mu$m – a combination of optical and terahertz frequencies respectively. Relativistic energies were chosen as the laser pulse durations shift more appreciably for such energies. The terahertz pulse was restricted to an intensity FWHM duration of $\tau_{fwhm,2} = 1$ ps, or a single cycle.

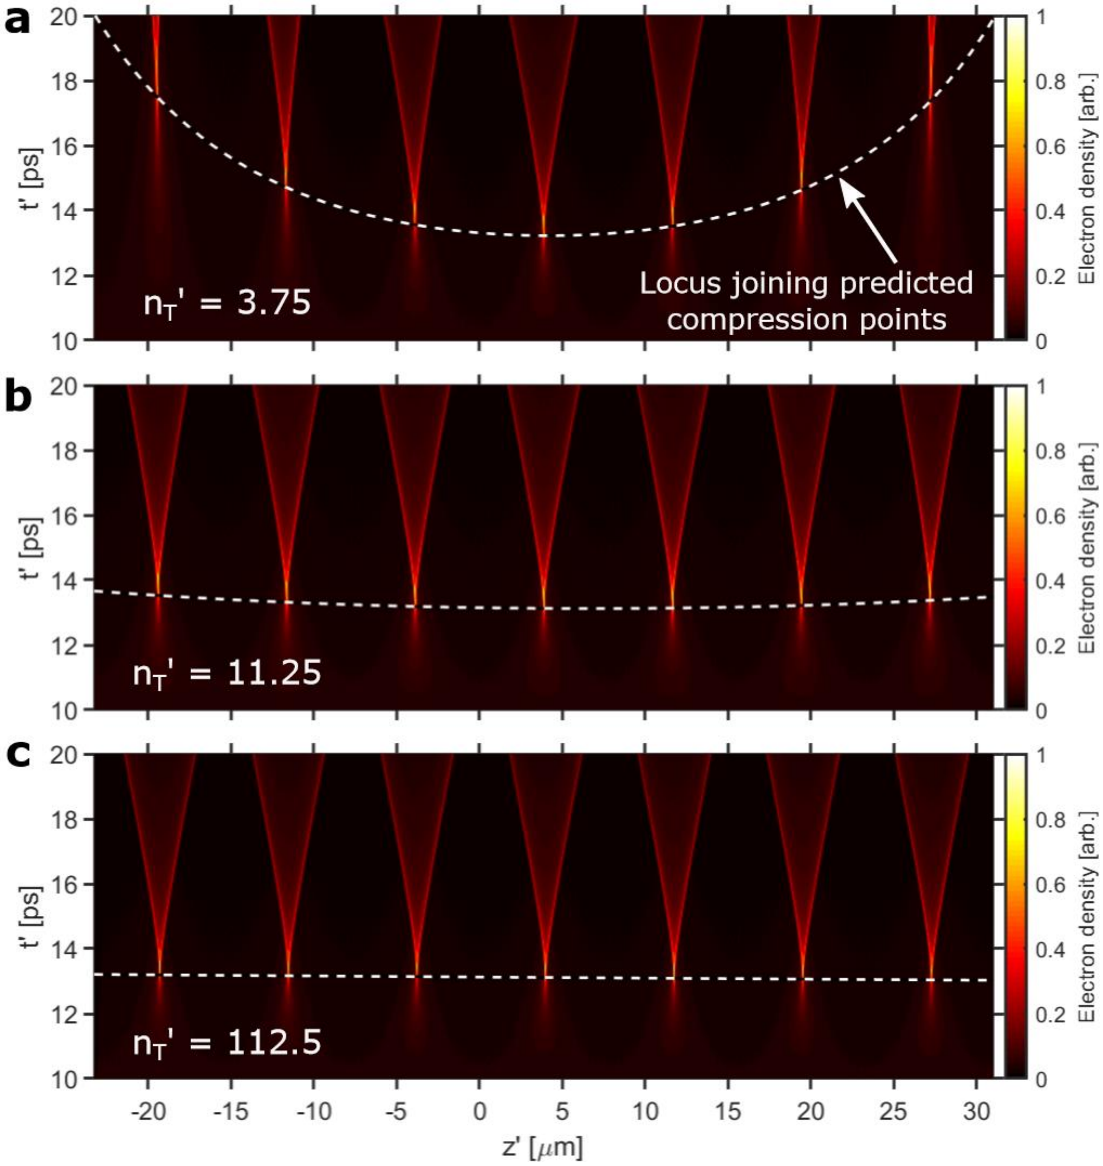


**Figure S5: Variation of compression times across multiple ponderomotive potential wells in the primed frame for 4.45 MeV electrons.** The electron bunch was compressed by counter-propagating optical and terahertz frequencies. The peak field strengths used were $E_{01} = 1 \times 10^{10}$ V/m and $E_{02} = 6 \times 10^{7}$ V/m. The counter-propagating terahertz wave intensity FWHM duration was kept constant at $\tau_{fwhm,2} = 1$ ps. The co-propagating optical wave FWHM duration take on three values: (a) $\tau_{fwhm,1} = 10$ fs, (b) $\tau_{fwhm,1} = 30$ fs, and (c) $\tau_{fwhm,1} = 300$ fs. The black-white dashed lines are the loci joining all predicted points of compression, given by Eq. (S56), when $z'_{min}$ is extended to the continuous domain containing all $z'_0$ values.

The optical pulse was varied over three values: $\tau_{fwhm,1} = 10$ fs, 30 fs, and 300 fs, corresponding to the following values for the pulse duration ratio in the same order: $n'_T = \tau'_{fwhm,1}/\tau'_{fwhm,2} = 3.75$, 11.25, and 112.5. The field strengths used were $E_{01} = 1 \times 10^{11}$ V/m and $E_{02} = 6 \times 10^{8}$ V/m. As Eq. (S56) indicates, a change in $T'_1$ or $T'_2$ would result in a change

in $\Delta t'_{foc}$ when $z'_0 \neq z'_{OL}$. Due to a quadratic dependence of the exponential term's argument on $(z'_0 - z'_{OL})$, when $T'_2$ is held constant, an increasing ratio, $n'_T = T'_1/T'_2$ would result in a broadening of the locus joining the predicted compression points (black-white dashed line). It can be observed that the predicted change in $\Delta t'_{foc}$ as a function of distance away from the central well is in good agreement with our numerical results. The focal time in the central well changes by only $\approx 0.1$ ps, or less than 5%, indicating the relative insensitivity of $\Delta t'_{foc}$ with respect to the changes in pulse durations for the central well. The knowledge of such multi-well compression time variation is useful for selection of pulse parameters which ensure optimal compression at the sample location.

In summary, we have used a perturbative method to derive approximate, closed-form asymptotic primed frame longitudinal trajectories. We have used this expression to derive the primed frame time separating interaction and maximum compression (focal time) being reached. Our inclusion of Gaussian envelopes show that focal times of the final bunches depend on their location with respect to the overlap position of the laser pulse peaks and the initial electron bunch. Knowledge of how this variation scales with the various laser parameters is crucial for ensuring the maximum possible compression is attained at the sample surface. We have shown that our predictions agree well with numerical simulations.

## S.3 Dynamics of quasi-monoenergetic electrons in pulsed wave intensity gratings

While the studying electron bunches with vanishing longitudinal momentum spreads is useful for deriving the time to focus, given by Eq. (S56), it does not allow us to predict how key compression quantities such as resulting energy spread and final electron bunch duration scale with the laser pulse parameters used and initial electron kinetic energy spread. In this section, we use the perturbative technique previously introduced to derive analytical first-order longitudinal primed frame trajectories. We then obtain theoretical scaling curves of the final electron bunch FWHM duration, resultant energy spread, and focal time versus the field strengths used and initial kinetic energy spread. We validate our results through numerical simulations and show that the predicted and exact values perfectly overlap.

Consider the primed frame zeroth-order transverse trajectories:

$$x'^{(0)}(t') = \beta'_{x,i} c t' + x'_0 \,, \tag{S58}$$

and

$$y'^{(0)}(t') = \beta'_{y,i}ct' + y'_0 \,. \tag{S59}$$

We have denoted the initial (at $t'_0 = 0$) $x$ and $y$ positions as $x'_0$ and $y'_0$, and the initial velocities as $\beta'_{x,i}c$ and $\beta'_{y,i}c$. For the longitudinal zeroth-order trajectory, we have:

$$z'^{(0)}(t') = \beta'_{z,i}ct' + z'_0 = \beta'_{z,i}c(t' - t'_{OL}) + z'_{OLe} \,, \tag{S60}$$

Where $\beta'_{z,i}c$ is the initial electron primed frame longitudinal velocity and $z'^{(0)}(t' = t'_{OL}) = z'_{OLe}$ is the primed frame electron longitudinal position at the time when the pulse peaks overlap, $t' = t'_{OL}$. We have chosen express (S60) using $z'_{OLe}$ instead of the initial position $z'^{(0)}(t' = 0) = z'_0$ since we wish to determine the ponderomotive deflection of the electron as a function of its initial velocity and position when the interaction with the grating occurs. It should be noted that this is consistent with our derivation in section S.2, where for a stationary electron in the primed frame, $z'_{OLe} = z'_0$. The same assumption of non-relativistic primed frame dynamics, both initial and resultant (as in sections S.1 and S.2) is in place: $\beta'_x, \beta'_y, \beta'_z \ll 1$, and $\beta' = \sqrt{{\beta'_x}^2 + {\beta'_y}^2 + {\beta'_z}^2} \ll 1 \Rightarrow \gamma' = 1/\sqrt{1 - {\beta'}^2} \approx 1$, the only difference being $\beta'_{z,i} \neq 0$ in this case. We once again assume that longitudinal fields vanish. We substitute (S58) to (S60) into the non-relativistic Lorentz force equations of motion, (S25) to (S27), in order to solve for $z'^{(1)}(t')$ and $\dot{z}'^{(1)}(t')$ in the same manner as in section S.2. Prior to integrating with respect to $t'$, we first state the expression for the longitudinal primed frame acceleration:

$$\begin{aligned}\ddot{z}'(t') = -\frac{e^2 {E'_{01}}^2}{m_e^2 c\omega'} \Bigg\{ & \frac{1}{2}{\mathcal{G}'_1}^2 \sin 2\eta'_1 + \frac{n'^2}{2}{\mathcal{G}'_2}^2 \sin 2\eta'_2 \\ & - n'\mathcal{G}'_1\mathcal{G}'_2 \cos\Delta\theta' \cos\left[2\beta'_{z,i}\omega'(t' - t'_{OL})\right] \sin(2k'z'_{OLe} + \phi'_{01} + \phi'_{02}) \\ & - n'\mathcal{G}'_1\mathcal{G}'_2 \cos\Delta\theta' \sin\left[2\beta'_{z,i}\omega'(t' - t'_{OL})\right] \cos(2k'z'_{OLe} + \phi'_{01} + \phi'_{02}) \\ & + \left(C'_{v_x}\cos\theta_1 + C'_{v_y}\sin\theta_1\right)\mathcal{G}'_1 \cos\eta'_1 \\ & - \left(C'_{v_x}\cos\theta_2 + C'_{v_y}\sin\theta_2\right) n'\mathcal{G}'_2 \cos\eta'_2 \Bigg\}. \end{aligned} \tag{S61}$$

Since we have defined $\beta'_{z,i} \ll 1$, we perform a Taylor expansion of the terms $\cos[2\beta'_{z,i}\omega'(t' - t'_{OL})]$ and $\sin[2\beta'_{z,i}\omega'(t' - t'_{OL})]$ up to second order with respect to some small deviation from $\beta'_{z,i} = 0$:

$$\cos[2\beta'_{z,i}\omega'(t'-t'_{OL})] \approx 1 - 2\omega'^2(t'-t'_{OL})^2{\beta'_{z,i}}^2 \,, \tag{S62}$$

$$\sin[2\beta'_{z,i}\omega'(t'-t'_{OL})] \approx 2\omega'(t'-t'_{OL})\beta'_{z,i} \,. \tag{S63}$$

Similar to section S.2, we are searching for asymptotic solutions to the equations of motion which, as we have seen, arise out of error functions in $t'$. As it turns out, an integration of (S61) with respect to $t'$ (up to some constant translation, $t'_{OL}$) after substituting back in the expanded terms (S62) and (S63), and invoking approximation (S36), yields Gaussian terms in $t'$for all terms of order 1 or higher in $t'$. As such, we know that in the limit $t' \gg t'_{OL}$, these terms do not survive and hence do not contribute to the asymptotic solutions. We thus omit them when stating the first-order longitudinal velocity for simplicity and compactness:

$$\begin{aligned}\dot{z}'^{(1)}(t') \approx -\frac{e^2{E'_{01}}^2}{m_e^2 c}\Bigg[&\frac{1}{4\omega'^2(1-\beta'_{z,i})}{\mathcal{G}'_1}^2\cos 2\eta'_1 - \frac{n'^2}{4\omega'^2(1+\beta'_{z,i})}\mathcal{G}'^2_2\cos 2\eta'_2 \\ &-\left(C'_{v_x}\cos\theta_1 + C'_{v_y}\sin\theta_1\right)\frac{1}{\omega'^2(1-\beta'_{z,i})}\mathcal{G}'_1\sin\eta'_1 \\ &-\left(C'_{v_x}\cos\theta_2 + C'_{v_y}\sin\theta_2\right)\frac{n'}{\omega'^2(1+\beta'_{z,i})}\mathcal{G}'_2\sin\eta'_2 \\ &-\Lambda\sin(2k'z'_{OLe}+\phi'_{01}+\phi'_{02})\,\mathrm{Erf}\left(\frac{2\alpha_a t' + \alpha_b}{2\sqrt{\alpha_a}{T'_1}^2}\right) + C'_{v_z}\Bigg].\end{aligned} \tag{S64}$$

We have once again defined the term $\Lambda$ to be:

$$\begin{aligned}\Lambda &= \frac{n'T'_1}{2\omega'}\sqrt{\frac{\pi}{\alpha_a}}\cos\Delta\theta\,\exp\left(\frac{\alpha_b^2 - 4\alpha_a\alpha_c}{4\alpha_a T'^2_1}\right) \\ &= \frac{n'T'_1}{2\omega'}\sqrt{\frac{\pi}{\alpha_a}}\cos\Delta\theta\,\exp\left\{\frac{-4(z'_{OLe}-z'_{OL})^2}{c^2[{T'_1}^2(1+\beta'_{z,i})^2 + {T'_2}^2(1-\beta'_{z,i})^2]}\right\}.\end{aligned} \tag{S65}$$

The terms $\alpha_a$, $\alpha_b$, and $\alpha_c$, also obey Eq. (S43):

$$\alpha_a = (1-\beta'_{z,i})^2 + \frac{T'_1}{T'_2}(1+\beta'_{z,i})^2 \,, \tag{S66}$$

$$\begin{aligned}\alpha_b = \frac{2}{c}\Bigg[&\frac{{T'_1}^2}{{T'_2}^2}\left(z'_{OLe} - z'_{i,2} - \beta'_{z,i}ct'_{OL}\right)(1+\beta'_{z,i}) \\ &-\left(z'_{OLe} - z'_{i,1} - \beta'_{z,i}ct'_{OL}\right)(1-\beta'_{z,i})\Bigg],\end{aligned} \tag{S67}$$

$$\alpha_c = \frac{1}{c^2}\left[\left(z'_{OLe} - z'_{i,1} - \beta'_{z,i} c t'_{OL}\right)^2 + \frac{T_1'^2}{T_2'^2}\left(z'_{OLe} - z'_{i,2} - \beta'_{z,i} c t'_{OL}\right)^2\right] . \tag{S68}$$

Equations (S66) to (S68) reduce to (S44) to (S46) in the case where $\beta'_{z,i} = 0$, and $z'_{OLe} = z'_0$. We evaluate (S64) in the limit $t' \gg t'_{OL}$, which gives the asymptotic longitdinal, primed frame velocity:

$$\frac{\dot{z}'^{(1)}(t' \gg t'_{OL})}{c} = \frac{\dot{z}'_f}{c} = \beta'_{z,f} = 2\Lambda \frac{e^2 {E'_{01}}^2}{m_e^2 c^2} \sin(2k' z'_{OLe} + \phi'_{01} + \phi'_{02}) + \beta'_{z,i} . \tag{S69}$$

When expanded, (S69) becomes Eq. (3) in the main text. The corresponding primed frame longitudinal trajectory in the $t' \gg t'_{OL}$ limit is:

$$\begin{aligned} z'^{(1)}(t' \gg t'_{OL}) &= z'_f(t') \\ &= \beta'_{z,f} c t' + z'_{OLe} - \beta'_{z,i} c t'_{OL} + \Lambda \frac{\alpha_b}{\alpha_a} \frac{e^2 {E'_{01}}^2}{m_e^2 c} \sin(2k' z'_{OLe} + \phi'_{01} + \phi'_{02}) . \end{aligned} \tag{S70}$$

When fully expanded, (S70) becomes Eq. (5) in the main text. Once again, setting the error function argument in (S64) to be 0 at $t'_{center}$ to find $z'_{center}$ at $t' = t'_{center}$, we get the principal temporal plane, which is also the center of interaction:

$$c t'_{center} = c t'_{OL} + (z'_{OLe} - z'_{OL}) \left[\frac{(1 - \beta'_{z,i}) T_2'^2 - (1 + \beta'_{z,i}) T_1'^2}{\left(1 - \beta'_{z,i}\right)^2 T_2'^2 + \left(1 + \beta'_{z,i}\right)^2 T_1'^2}\right] . \tag{S71}$$

When evaluated at $\beta'_{z,i} = 0$ and $z'_{OLe} = z'_0$, (S71) reduces to (S50).

We can use (S69) and (S70) to determine theoretical values of compression quantities such as FWHM bunch duration and final kinetic energy spread. We do this by considering $N$ electrons in the central well. $N$ values of $z'_{OLe}$ were initialized in the primed frame following a uniform random distribution, which is valid if the entire electron bunch length is much larger than a single ponderomotive grating period and the longitudinal rest frame phase space particle distribution is uncorrelated. For a given lab frame dimensionless energy spread, which we take to be the standard deviation (SD), $\sigma_\gamma$, we can obtain the normalized momentum spread, $\sigma_{\gamma\beta}$ through the relation (see Section S.5(iii)):

$$\beta_0 \sigma_{\gamma\beta} = \sigma_\gamma . \tag{S72}$$

The mean dimensionless bunch velocity in the lab frame is $\beta_0$ for our bunch propagating in $+z'$. Assuming the mean transverse momenta vanish, which is typically the case, the mean

normalized momentum will be $\gamma_0\beta_0$, and the spread will be $\sigma_{\gamma\beta} = \sigma_{\gamma\beta_z}$. The transverse extent is irrelevant since we are considering the plane wave limit. The transverse momentum spread is assumed to be unchanged during interaction, which has been experimentally shown to be true in the absence of space charge [4]. The momentum distribution was initialized in the lab frame, and $\beta'_{z,0}$ is obtained from $\beta_{z,0}$ through the relativistic velocity addition formula:

$$\beta'_{z,i} = \frac{\beta_{z,i} - \beta_0}{1 - \beta_0\beta_{z,i}} \, . \tag{S73}$$

Together with the Lorentz-transformed laser pulse parameters, $\beta'_{z,i}$ and $z'_{OLe}$ are then fed into (S70) to obtain a set of primed frame trajectories. The FWHM bunch spatial width in the primed frame, $\Delta z'$, is then computed using linear interpolation of the discrete spatial distribution at each time step. The lab frame FWHM duration above background is then obtained from $\tau_e = \Delta z'/\gamma_0\beta_0 c$. The background is defined to be the average of the particle count at the extreme edges of the well since the regions in the vicinity of the grating maxima do not impart significant forces on the electrons there. Also, these electrons do not contribute to the formation of the high-density bunch core. The only non-analytical portion of our formulation is the randomly-generated particle position-momentum distributions at the time of interaction. It should be noted that multiple gratings periods can also be modelled by changing the $z$-spatial distribution and range at initialization. However, for our purposes, which is to investigate the scaling of compression quantities of electrons in a single grating period at interaction, we restrict the initialization values to the central well where compression is the strongest. It should be noted that $N$ should be large enough such that the spatial distribution at each time step becomes almost continuous.

Figure S6 shows a comparison between the numerical results (plane wave simulations, no space charge) and our theoretical predictions. The numerical simulations were carried out in the lab frame with $3.75 \times 10^5$ non-interacting electrons of 5 MeV mean kinetic energy, $\langle \mathrm{E_K} \rangle$, and 0.14% initial relative $E_K$ SD, $\sigma_{\mathrm{E_K}}/\langle \mathrm{E_K} \rangle$. Electrons of this mean $E_K$ are velocity-matched by counter-propagating lasers of wavelengths $\lambda_1 = 0.65\ \mu$m and $\lambda_2 = 300\ \mu$m. The field amplitudes used are: $E_{01} = 1 \times 10^{11}$ V/m and $E_{02} = 2 \times 10^8$ V/m. The intensity FWHM durations of the pulses are $\tau_{fwhm,1} = 30$ ps and $\tau_{fwhm,2} = 1$ ps. In the absence of all fields, the electrons are uncorrelated in longitudinal phase space at the time of interaction and occupy exactly one grating period following a uniform random distribution. At this time, the momenta are normally distributed in all directions. The theoretical results were obtained using $N = 10^6$

electrons. Our theoretical predictions are in perfect agreement with numerically-obtained values: the predicted minimum FWHM bunch duration is 366 as while the numerically-computed value is 378 as. The predicted time between the interaction center and the time when the minimum FWHM duration is obtained is 10.76 ps while the numerical result is 10.43 ps. The theoretically-predicted final $E_K$ SD is 0.310% while the numerical result is 0.308%.

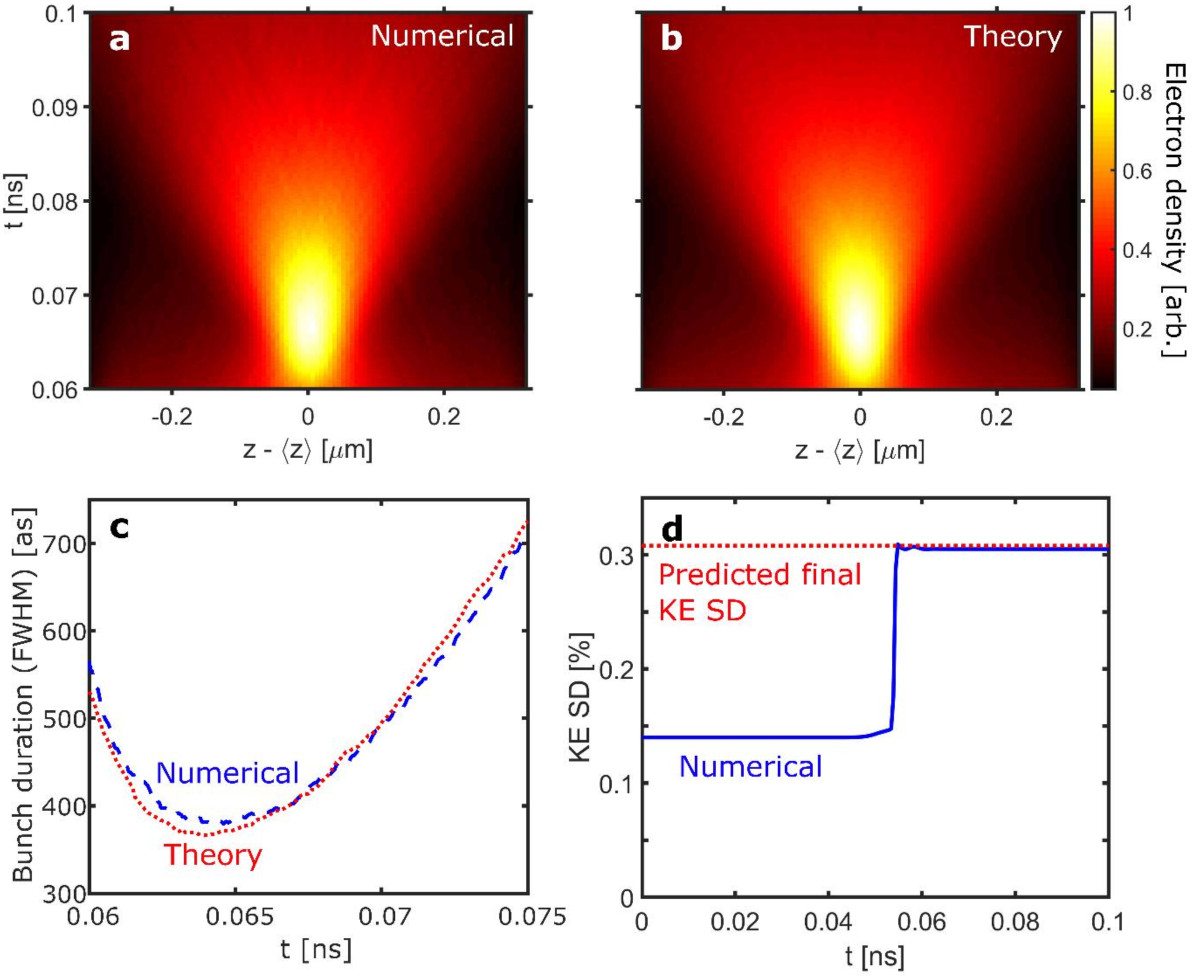


**Figure S6: Comparison between numerical results and theoretical values for the compression of 5 MeV electrons of 0.14% kinetic energy spread (SD).** (a) and (b) show the time-evolution of the electron density in the central well for the numerical and theoretical cases respectively. The time-evolution of the FWHM duration for both cases are plotted in (c). The time-evolution of the kinetic energy SD is depicted in (d), with the predicted final $E_K$ SD value overlaid. The spatial distribution of the electrons at the minimum FWHM duration is plotted in figure S7(f). The parameters used to produce these plots are: $E_{01} = 1 \times 10^{11}$ V/m, $E_{02} = 2 \times 10^{8}$ V/m, $\tau_{fwhm,1} = 30$ fs, $\tau_{fwhm,2} = 1$ ps. The initial lab frame momentum spread is isotropic in $x$, $y$, and $z$. The transverse momentum is assumed to be unchanged for the theoretical case. The simulations were carried out in the plane wave limit.

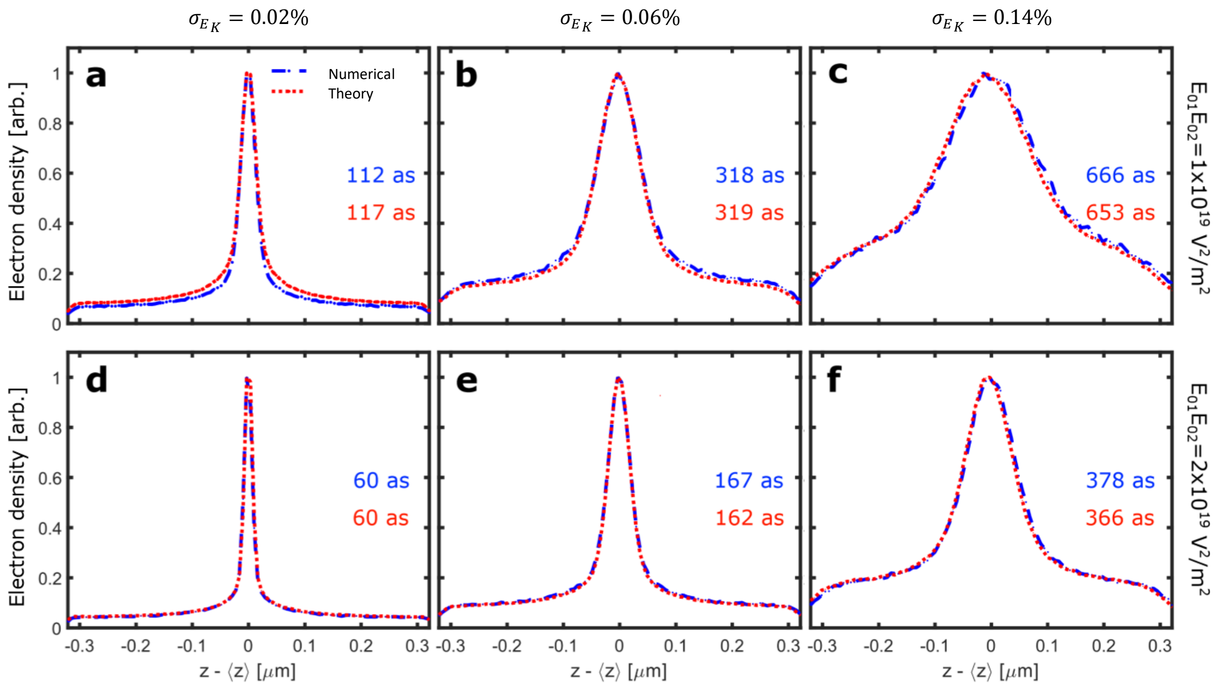


**Figure S7: Comparison between the numerically-computed and theoretically-predicted spatial electron distributions at the time of minimum FWHM duration.** Numerical simulations were carried out with 5 MeV electron bunches in the lab frame. The left, middle, and right panel columns show results for lab frame kinetic energy spreads (SD) of 0.02%, 0.06%, and 0.14% respectively. The top and bottom row of panels correspond to results stemming from the use of combined field amplitudes $E_{01}E_{02} = 1 \times 10^{19}\ \mathrm{V}^2/\mathrm{m}^2$ and $E_{01}E_{02} = 2 \times 10^{19}\ \mathrm{V}^2/\mathrm{m}^2$ respectively. $E_{01}$ was kept constant at $E_{01} = 1 \times 10^{11}$ V/m. In all cases, the laser pulse intensity peaks overlap with each other in the centre of the grating period. The laser pulse intensity FWHM durations used are: $\tau_{fwhm,1} = 30$ fs and $\tau_{fwhm,2} = 1$ ps. The blue dashed lines and red dotted lines show the lab frame spatial distribution obtained numerically and theoretically in that order. The minimum FWHM bunch durations are labelled in each panel with the same colour scheme. The theoretical spatial distributions overlap almost perfectly with the numerical ones.

The electron bunch used had 5 MeV mean $E_K$. Three different $E_K$ SD values were used: $\sigma_{\mathrm{E_K}}/\langle \mathrm{E_K} \rangle = 0.02\%, 0.06\%,$ and $0.14\%$ were used to produce the left, middle, and right columns of figure S7 respectively. Once again, isotropic normalized momentum spreads (SD) in $x, y,$ and $z$ were used. The lab frame values corresponding to the aforementioned energy spread values in the same order are: $\sigma_{\gamma\beta_i} = 1.9615 \times 10^{-3}, 5.8848 \times 10^{-3}$, and $1.3733 \times 10^{-2}$, where $i \in \{x, y, z\}$. For all cases, $E_{01} = 1 \times 10^{11}$ V/m was used. The laser pulse intensity FWHM durations were $\tau_{fwhm,1} = 30$ fs and $\tau_{fwhm,2} = 1$ ps. The top row of panels correspond to the counter-propagating laser peak field amplitude $E_{02} = 1 \times 10^{8}$ V/m while the bottom panels correspond to $E_{02} = 2 \times 10^{8}$ V/m. It can be seen that the theoretical

distributions, plotted using $10^6$ electrons, almost perfectly overlap the numerally-obtained ones in the plane wave limit. This shows that our asymptotic trajectory equations, when combined with large-enough, randomly generated values of position and momentum of a desired distribution at the time of interaction, replicates the exact electrodynamic interaction very closely. In the main text, other values of electron mean $E_K$, energy spreads, as well as laser pulse parameters have been used to validate our method of predicting FWHM values, resultant energy spreads, and focal time in both the plane wave and non-paraxial limits.

In summary, we have used a perturbative technique, similar to that in section S.2, in order to derive the primed frame trajectories for a quasi-monoenergetic, non-interacting electron bunch. Coupled with a user-specified electron bunch configuration at the time of interaction, our analytical expressions can be used to predict quantities of interest such as the time when the minimum attosecond bunch duration is attained (focus), minimum FWHM duration at the focus, and the resultant energy spread when given a specified energy spread and a set of laser pulse parameters. Using our method, these quantities can be predicted with great accuracy. We have validated our predictions with plane EM wave simulations and have plotted a few select cases here with more results shown in the main text.

## S.4 Limitations of analytical formulation

In this section, we summarize the assumptions which enabled us to derive closed-form, expressions for the electron velocity and position long after interacting with the intensity grating. We briefly discuss the possible limitations which stem from the assumptions we have made. We also discuss the effect of how disproportionate amplitudes in the primed frame can hamper compression of electron bunches.

In deriving the closed-form expressions for the final primed frame velocity, $\dot{z}'_f$, and longitudinal position, $z'_f(t')$, long after the electron-intensity grating interaction (for both in the $\beta'_{z,i} = 0$ and $\beta'_{z,i} \neq 0$ cases), we made a total of 6 assumptions. We can summarise them as such:

1. The laser pulses considered can be approximated as pulsed plane waves
2. All laser pulses a have Gaussian frequency spectrum
3. The electron bunch $E_K$ spread is small enough such that the non-relativistic Lorentz force equation is valid in the primed frame.

4. Space charge effects can be neglected.
5. Maximum electron bunch compression (focus) is attained when the electrons are not subjected to any forces.

Assumptions 2-4 are generally quite valid. For assumption 2 (Gaussian frequency spectrum), despite using a single-cycle terahertz pulse for all relativistic simulations, modelled accurately using a Poisson power spectrum, we find that theoretical predictions agree well with the numerical simulations (main text figure 3), especially in the plane wave limit. Assumption 3 (validity of the non-relativistic Lorentz force equation in the primed frame) is valid for small relative kinetic energy spreads; we restrict the values considered to $< 1\%$, which is representative of realistic few-MeV electron bunches. Assumption 4 (negligible space charge effects) holds in the single-electron and relativistic limits.

Assumptions 1 and 5 are the most likely to cause discrepancies. Assumption 1 (pulsed plane wave profiles) holds when the laser beam waist is much larger than the transverse extent of the electron bunch. As we have seen from figure 3 in the main text, in the strongly non-paraxial regime, finite beam waists give rise to weaker-than-predicted compression, which is pronounced even for beam waists 30 times larger than the electron bunch radius. However, the theoretical formulations still provide valid order-of-magnitude estimates (including scaling trends) for compression quantities such as the FWHM bunch duration, the focal time, and the final $E_K$ spread of the bunch.

Assumption 5 (maximum compression occurring when the electrons do not experience any forces) is a key assumption that places limits on the validity of the formulation. This assumption is required because the asymptotic solutions are evaluated in the limit when $t' \gg t'_{center}$ (and also $t' \gg t'_{OL}$), and the solutions were used to predict the focal time, given by Eq. (S56). Hence, our formulation breaks down when maximum compression is attained during the time when the forces imparted by the grating are still significant. This is clearly shown and discussed in Section S.2.

We now briefly discuss and explore the effect of the co-propagating (primed) frame ratio of co-propagating to counter-propagating EM wave peak electric field strengths which our closed form expression for focal time do not account for. In the primed frame, greater symmetry between counter-propagating pulses is favoured. In the absence of space charge and

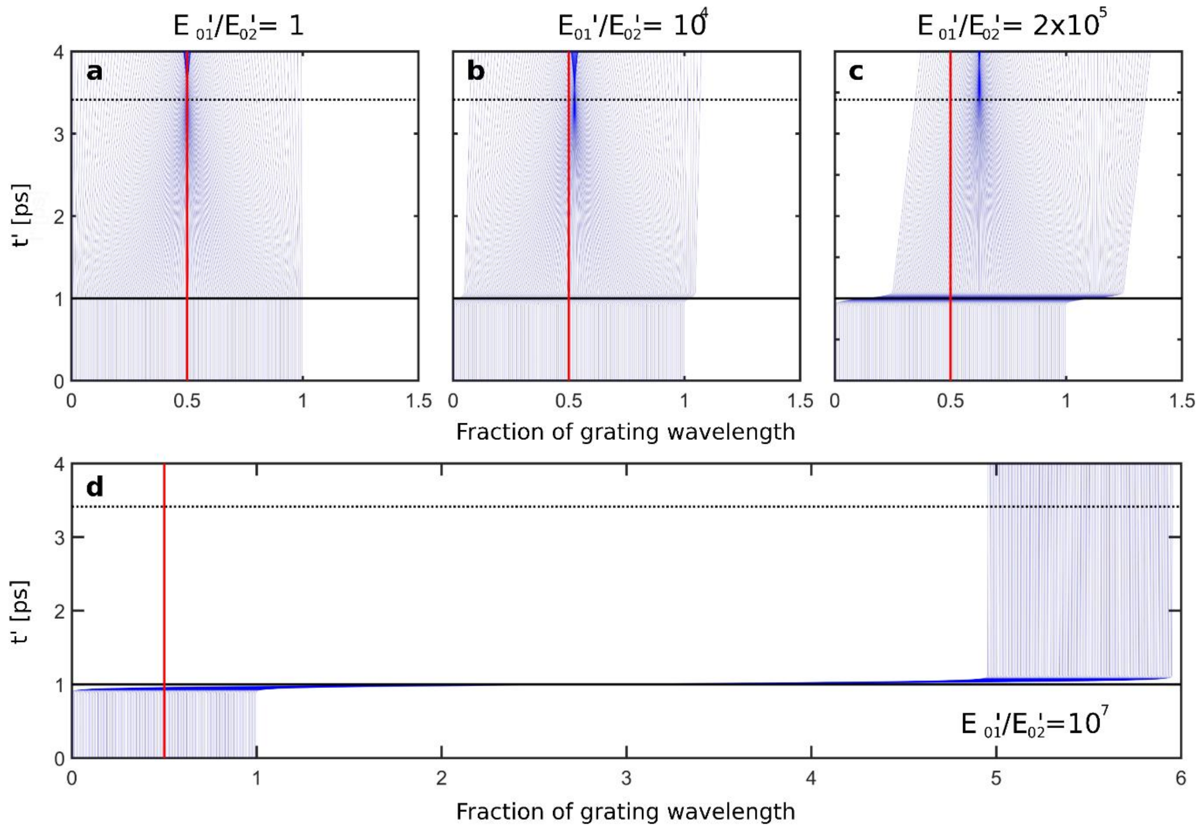


**Figure S8: Plots of numerically-computed electron trajectories with no space charge and initial velocity spread showing displacement of compression positions from the potential well minima in the primed frame for various $E'_{01}/E'_{02}$ values.** The solid, red vertical line coincides with the well minimum position, which is the expected point of compression. The solid and dotted horizontal black lines denote the interaction time and expected time of maximum compression respectively. (a) For the case of equal primed frame durations and amplitudes, the primed frame compression location coincides with the well minimum exactly. (b) and (c) Significant shifts (>1%) in compression point from the well minimum occur for $E'_{01}/E'_{02} \geq 10^4$. (d) For extremely large disparities between the co-propagating and counter-propagating EM wave electric field strength amplitudes, e.g. $E'_{01}/E'_{02} = 10^7$, compression no longer takes place.

velocity spread, the ideal compression scenario would be the formation of a bunch centred exactly at the well minimum. This only occurs if the primed frame durations and intensities are exactly equal. However, this may be hard to achieve, especially in the relativistic regime where durations and field strengths transform drastically between the lab and primed frames. Effects of great imbalances between counterpropagating wave parameters would result in effects such as phase mismatch between the grating and the bunch formation location. For instance, if both pulses are of similar primed frame duration, but one pulse has a peak field strength many orders of magnitude greater than the other, the point of compression would shift and the bunches

formed are no longer centred at the minima. If the disparity is large enough compression into a train of sub-fs bunches do not occur.

Our previous derivations of focal time in the primed frame, Eq. (S56), assumes that compression always takes place at the minimum of each ponderomotive well and does not account for changes caused by ratio $E'_{02}/E'_{01} \neq 1$. With reference to figure S8, which shows numerically-computed trajectories of varying $E'_{02}/E'_{01}$ values but constant $E'_{01}E'_{02}$ and primed frame pulse duration values, it can be seen that this is not the case. The solid, red vertical lines, coinciding with the position of the well minimum, show the expected position of compression within the ponderomotive well (in the primed frame). The solid and dotted horizontal black lines denote the times of electron-grating interaction and expected maximum compression respectively. For ratios $E'_{01}/E'_{02} \leq 10^3$, the shift in the primed frame longitudinal coordinate, $z'$, from the well minimum position as a percentage of a single grating period is less than 1%. For $E'_{01}/E'_{02} \geq 10^4$, the shifts become more significant (Figures. S8(b) and (c)). Should the ratio of field strengths become extremely large, e.g. $E'_{01}/E'_{02} = 10^7$ (figure S8(d)), compression does not occur at all, and all the electrons are pushed out of the ponderomotive well. Thus, when choosing parameters, it would be best if the electric field amplitudes of the counter-propagating waves were equal in the rest frame of the electron. For all the cases we have considered both in the main text and the supporting information, the primed frame amplitudes are within an order of magnitude of each other, yielding shifts which are negligible.

## S.5 Methods and parameters used in main text

### S.5 (i) Numerical integration of the equations of motion

Numerical simulations of the electron-laser interaction were carried out by solving the Newton-Lorentz equations of motion:

$$\frac{d(\gamma\vec{\beta})}{dt} = \frac{q}{mc}\left(\vec{E} + \vec{\beta}c \times \vec{B}\right). \tag{S74}$$

The electric and magnetic field vectors are denoted as $\vec{E}$ and$\vec{B}$. The $\vec{E}$, and $\vec{B}$ we use are finite-energy, exact, closed-form solutions to Maxwell's equations for non-paraxial pulses. The dimensionless velocity vector is $\vec{\beta}$, and the corresponding Lorentz factor is $\gamma = 1/\sqrt{1-\beta^2}$ . The charge and rest mass of the simulated charged particle are $q$ and $m$ respectively, and the

speed of light in free space is $c$. The numerical integration was carried out by implementing a fifth-order, adaptive step Runge-Kutta algorithm.

The pair-wise space charge interactions between all electrons were computed using exact expressions for both near- (velocity dependent and responsible for the Coulomb force) and far-fields (acceleration dependent and associated with the electron radiation) obtained from the Lienard-Wiechert potentials. Our simulations also took into account radiation reaction via the Landau-Lifshitz formula, but we have verified that radiation reaction has negligible effect in all scenarios studied in the paper. For more details of our algorithm, see the Supplementary Information in [5] and [6].

### S.5 (ii) Exact, finite-energy, pulsed solutions to Maxwell's equations

As the terahertz pulses we use are focused down to dimensions close to the size of the central wavelength and are single-cycle, non-paraxial effects, such as non-vanishing and non-neglible longitudinal fields, arise. In order to accurately incorporate fully non-paraxial pulses, we adopt the method used in [7] to construct exact, finite-energy, closed-form solutions to Maxwell's equations as opposed to the paraxial wave equation. Expressed in terms of the electric and magnetic Hertz vector potentials, $\vec{\Pi}$ and $\vec{\Pi}^*$ respectively, the field expressions are given by [8]:

$$\vec{E} = Re\left[\nabla \times \left(\nabla \times \vec{\Pi}\right) - \nabla \times \mu_0 \partial_t \vec{\Pi}^*\right] \tag{S75}$$

$$\vec{B} = Re\left[\mu_0 \nabla \times \left(\nabla \times \vec{\Pi}^*\right) + \epsilon_0 \mu_0 \nabla \times \partial_t \vec{\Pi}\right] \tag{S76}$$

where $Re[\,]$ denotes taking the real part of the complex fields. The Hertz vector potentials corresponding to a non-paraxial pulse, linearly-polarized in $x$ are [7]:

$$\vec{\Pi} = \hat{x}\Psi(x, y, z, t) \tag{S77}$$

$$\vec{\Pi}^* = \hat{y}c\epsilon_0\Psi(x, y, z, t). \tag{S78}$$

The free space electric permittivity and magnetic permeability are denoted $\epsilon_0$ and $\mu_0$ respectively. The speed of light in free space is defined such that $\epsilon_0\mu_0 = 1/c^2$. The phasor, $\Psi(x, y, z, t)$, which incorporates a Poisson power spectrum [3], has the following form

$$\Psi(x, y, z, t) = \frac{\Psi_0 \exp(i\phi_0)}{\tilde{R}} [f(t_+)^{-s-1} - f(t_-)^{-s-1}]. \tag{S79}$$

This phasor is valid in the sub-cycle and multi-cycle limits, and does not have unphysical negative frequencies. We have defined

$$f(t_\pm) = 1 - \frac{i\omega_0}{s}\left(t \pm \frac{\tilde{R}}{c} + i\frac{a}{c}\right). \tag{S80}$$

We have denoted the constant amplitude as $\Psi_0$, some constant phase shift as $\phi_0$, the central angular frequency as $\omega_0$, a real-valued, positive Lorentz invariant controlling the pulse duration as $s$, the real-valued confocal parameter controlling the beam waist as $a$, and $\tilde{R} = \sqrt{x^2 + y^2 + (z + ia)^2}$. The imaginary unit is $i = \sqrt{-1}$.

### S.5(iii) Initial electron phase space distribution

The electron bunches were initialized in the lab frame at transverse and longitudinal waists (minimum transverse and longitudinal extent) where the deviation of each momentum and sptial component from the mean ($\gamma\beta_i - \langle\gamma\beta_i\rangle$, where $i \in \{x, y, z\}$, and $\vec{r} - \langle\vec{r}\rangle$ where $\vec{r} = (x, y, z)$) are uncorrelated. The $x$- and $y$-coordinates were initialized with a Gaussian distribution with equal standard deviations (SD) $\sigma_x = \sigma_y$, which we define to be the bunch waist radius, and centered on the propagation axis, $\langle x\rangle = \langle y\rangle = 0$. We initialized the momentum components with a Gaussian distribution in $\gamma\beta_x$, $\gamma\beta_y$, and $\gamma\beta_z$. The mean momenta were $\langle\gamma\beta_x\rangle = \langle\gamma\beta_y\rangle = 0$, and $\langle\gamma\beta_z\rangle = \gamma_0\beta_0$, where $\beta_0$ corresponds to the bunch central velocity and $\gamma_0 = 1/\sqrt{1-\beta_0^2}$ is the corresponding Lorentz factor. For a differential absolute kinetic energy spread $\Delta\gamma$, the corresponding differential spread in the total momentum is:

$$\Delta(\gamma\beta) = \frac{\Delta\gamma}{\beta_0} \tag{S80}$$

In order to obtain a dependence of $\Delta(\gamma\beta)$ on the individual momentum components $\Delta(\gamma\beta_i)$ for $i \in \{x, y, z\}$, we take the derivative of $(\gamma\beta)^2$ with respect to $\gamma\beta$:

$$\frac{d(\gamma\beta)^2}{d(\gamma\beta)} = 2(\gamma\beta) \Rightarrow d(\gamma\beta) = \frac{d(\gamma\beta)^2}{2(\gamma\beta)}\ . \tag{S81}$$

Using the chain rule and expressing the total derivatives in terms of partial derivatives, we get:

$$d(\gamma\beta) = \frac{1}{2(\gamma\beta)} \sum_{i\in\{x,y,z\}} \frac{\partial(\gamma\beta)^2}{\partial(\gamma\beta_i)}\, d(\gamma\beta_i)$$
$$= \frac{1}{\gamma\beta}\left[\gamma\beta_x\, d(\gamma\beta_x) + \gamma\beta_y\, d\big(\gamma\beta_y\big) + \gamma\beta_z\, d(\gamma\beta_z)\right], \tag{S82}$$

where $(\gamma\beta)^2 = (\gamma\beta_x)^2 + \big(\gamma\beta_y\big)^2 + (\gamma\beta_z)^2$ . Once again, for small spreads away from the non-zero mean momenta components, we get:

$$\Delta(\gamma\beta) = \frac{1}{\gamma_0\beta_0}\left[\langle\gamma\beta_x\rangle\Delta(\gamma\beta_x) + \langle\gamma\beta_y\rangle\Delta\big(\gamma\beta_y\big) + \langle\gamma\beta_z\rangle\Delta(\gamma\beta_z)\right]. \tag{S83}$$

For the simplest case we consider, where the mean transverse momenta vanish and $\gamma_0\beta_0 \approx \langle\gamma\beta_z\rangle$ (and $\gamma_0\beta_0 \neq 0$), (S83) simplifies to

$$\Delta(\gamma\beta) = \Delta(\gamma\beta_z), \tag{S84}$$

And the transverse momenta can be initialized independently (to first order) of $\Delta(\gamma\beta)$ and $\Delta(\gamma\beta_z)$.

We assume all spreads to be the SD: $\Delta(\gamma\beta) = \sigma_{\gamma\beta}$, $\Delta(\gamma\beta_i) = \sigma_{\gamma\beta_i}$ for $i \in \{x, y, z\}$, $\Delta\gamma = \sigma_\gamma$. For a given $\sigma_\gamma$, we initialized the momenta components and computed the exact $\sigma_\gamma$ corresponding to the initialized momentum distributions until the initialized values of momentum and well as energy spread were within 0.01% of the desired values. In the main text, the relative KE spread, was defined to be $\sigma_\gamma/(\gamma_0 - 1) = \sigma_{\mathrm{KE}}/\langle\mathrm{KE}\rangle$.

To simulate transverse and longitudinal focusing of the initial electron bunch, each electron was traced back in time by some fixed interval in the absence of all forces. This corresponds to the bunch centroid $\langle z\rangle$ propagating in the negative $z$-direction. After this re-tracing procedure, the bunch acquires a negative velocity chirp in all directions, which is representative of a bunch leaving a focusing element. This is the new initial bunch with which each simulation is carried out. We time the interaction between the counter-propagating laser pulses and the electron bunch such that laser intensity pulse peaks coincide with each other and the electron bunch at the same time.

### S.5 (iv) Case 1 parameters: low-charge, low-KE spread electron bunch

In this section, we state in full the parameters used for the case of a low-charge, low-KE spread bunch. For a 5 MeV bunch, we have: $\beta_0 = 0.9956760$ and $\gamma_0 = 10.7649968$. The bunch charge simulated was 2 fC. In our simulations, 1250 macroparticles were used. The

electrons were initialized in $z$ following a random uniform distribution spanning $10\lambda_{gr}$. This truncated bunch simulates the central portion of an electron bunch which is long enough for the central bunch region to be approximately uniform in charge density (in $z$). The bunch radius when transverse waist is reached is $\sigma_x = \sigma_y = 15$ μm. The relative KE SD chosen was $\sigma_{\text{KE}}/\langle\text{KE}\rangle = 10^{-3}\%$, and assuming the bunch centroid propagates in only the $+z$-direction resulting in vanishing mean momenta in $x$ and $y$, this corresponds to a longitudinal momentum spread of $\sigma_{\gamma\beta_z} \approx 9.808 \times 10^{-5}$ For simplicity, we configured the bunch such that the momentum spread was isotropic: $\sigma_{\gamma\beta_x} = \sigma_{\gamma\beta_y} = \sigma_{\gamma\beta_z}$. The bunch distribution in each phase space plane was uncorrelated at initialization, as stated in the previous section using the parameters above. The bunch centroid was then propagated backward in time by $\Delta t = \gamma_0(10\text{ ps}) \approx 107.65$ ps in the absence of forces.

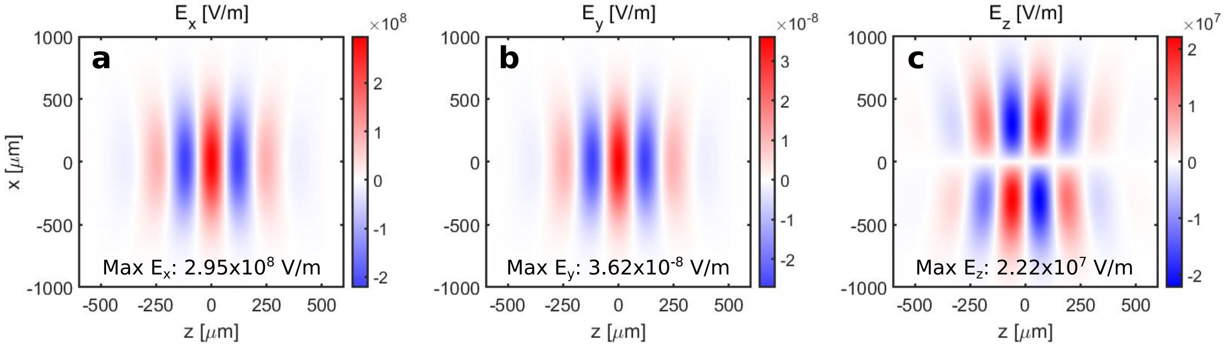


**Figure S9: Single-cycle terahertz electric field profile for case 1.** The plot shows the 1 THz wave ($\lambda = 300$ μm) centered at the point of focus. The intensity FWHM duration is 1 ps and the peak field strength in $x$ is about $2.95 \times 10^8$ V/m. The beam waist radius is 450 μm. The corresponding pulse energy is about 39 μJ.

For both laser pulses, we chose their focal points to coincide with each other, centered on-axis: $x_{foc} = y_{foc} = 0$ m at $z_{foc} \approx 3.217068 \times 10^{-2}$ m. The optical and terahertz pulse intensity peak positions relative to $z_{foc}$ at initial time $t = 0$ s were $z \approx -3.23101 \times 10^{-2}$ m and $z \approx 3.23101 \times 10^{-2}$ m respectively. Both beam waists were $w_0 = 450$ μm. The optical pulse intensity FWHM duration chosen was 80 fs. The terahertz pulse FWHM duration was 1 ps long. The on-axis peak field strengths of the optical and terahertz pulses at the focus are $E_{01} = 4.96 \times 10^{10}$ V/m and $E_{02} = 2.95 \times 10^8$ V/m respectively. Corresponding to these parameters, the optical and terahertz pulses have pulse energies of about 90.3 mJ and 39.0 μJ respectively. The terahertz electric field profiles in each direction are plotted in figure S9.

These parameters were also used to produce Figure 2 in the main text. Only the bunch charge and initial bunch KE were varied.

### S.5 (v) Case 2 parameters: 20 fC, 7 fs, 8 μm-radius electron bunch

In this section, we state all parameters used to create a 20 fC, 7 fs (SD) electron bunch with realistic properties as well as the laser pulse parameters chosen. We adapted the electron bunch parameters from reference [9] and assumed, for simplicity, that the momentum and spatial distributions were normally distributed in $x, y$, and $z$. From Figures 2(c) and 2(d) in [9], we estimated $\sigma_x = \sigma_y \approx 8$ μm, which we have defined to be our radius. The transverse emittance values given were $\epsilon_{x,rms,n} \approx 16$ nm rad and $\epsilon_{y,rms,n} \approx 20$ nm rad. We take the definition of the normalized, rms emittance to be

$$\epsilon_{x,rms,n} = \sqrt{\langle x^2\rangle\langle\gamma^2\beta_x^2\rangle - \langle x\gamma\beta_x\rangle^2}\,, \tag{S85}$$

where $\langle\ \rangle$ is the expectation value operator. Assuming the bunch is uncorrelated in phase space at the focus in all 3 phase space planes, the bunch is centered on-axis: $\langle x\rangle = \langle y\rangle = 0$, and the bunch centroid motion is confined to $z$: $\langle\gamma\beta_x\rangle = \langle\gamma\beta_y\rangle = 0$, we have $\epsilon_{x,rms,n} = \sigma_x\sigma_{\gamma\beta_x} =$ 16 nm rad and $\epsilon_{y,rms,n} = \sigma_y\sigma_{\gamma\beta_y} = 20$ nm rad. Using $\sigma_x = \sigma_y = 8$ μm, we have $\sigma_{\gamma\beta_x} =$ $2.0 \times 10^{-3}$ and $\sigma_{\gamma\beta_y} = 2.5 \times 10^{-3}$. From Figure 3(b) in [9], we estimate the longitudinal emittance to be $\epsilon_{z,rms,n} \approx 30$ nm rad. Once again assuming that this value corresponds to the longitudinal waist, where $\sigma_z = \sigma_{\tau_e}\beta_0 c$ and (SD bunch duration) $\sigma_{\tau_e}$ =7 fs, we have:

$$\epsilon_{z,rms,n} = \sigma_{\tau_e}\beta_0 c\sigma_{\gamma\beta_z} \Rightarrow \sigma_{\gamma\beta_z} \approx 1.4356 \times 10^{-2}\,. \tag{S86}$$

This corresponds to a relative KE SD of $\sigma_{\mathrm{KE}}/\langle\mathrm{KE}\rangle \approx 0.146\,\%$. Consistent with our assumption that the $z$-spatial distribution is also Gaussian, the bunch FWHM corresponding to $\sigma_{\tau_e} = 7$ fs is $2\sqrt{2\log 2}\,\sigma_{\tau_e} \approx 16.5$ fs, which is the value stated in the main text. The uncorrelated phase space bunch distribution at initialization was propagated back by a constant time interval of $\Delta t = \gamma_0(2.12\text{ ps}) \approx 22.82$ ps to simulate a bunch focusing transversally and longitudinally.

For both laser pulses, we once again chose their focii to coincide with each other and the interaction point, centered on-axis: $x_{foc} = y_{foc} = 0$ m at $z_{foc} \approx 6.849799 \times 10^{-3}$ m. The optical and terahertz pulse intensity peak positions relative to $z_{foc}$ at initial time $t = 0$ s are $z \approx -6.879220 \times 10^{-3}$ m and $z \approx 6.879220 \times 10^{-3}$ m respectively. The beam waists were

both chosen to be $w_0 = 200$ μm. The optical pulse intensity FWHM duration chosen was 30 fs. The terahertz pulse intensity FWHM duration chosen was 1 ps. The on-axis peak field strengths of the optical and terahertz pulses at the focus were $E_{01} \approx 5 \times 10^{10}$ V/m and $E_{02} \approx 4.18 \times 10^{8}$ V/m respectively. Corresponding to these parameters, the optical and terahertz pulses have energies of about 6.66 mJ and 16.9 μJ respectively. The terahertz electric field profiles in each direction are plotted in figure S10.

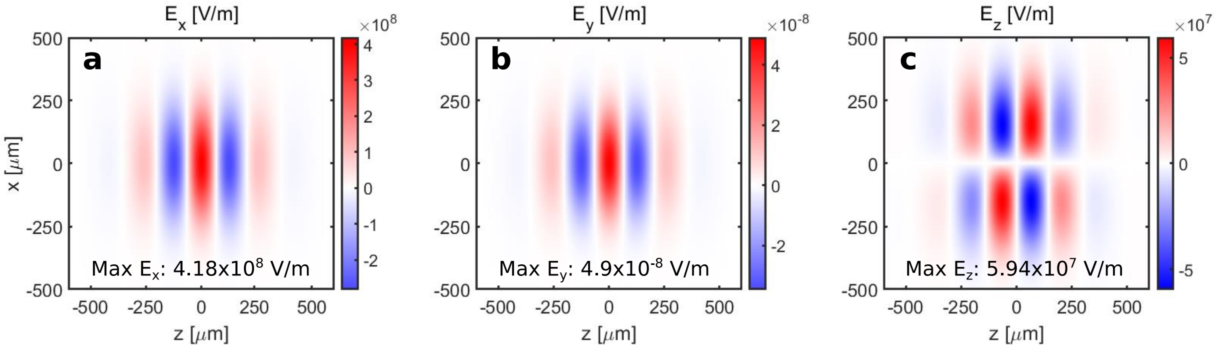


**Figure S10: Single-cycle terahertz electric field profile for case 2.** The plot shows the 1 THz wave ($\lambda = 300$ μm) centered at the point of focus. The intensity FWHM duration is 1 ps and the peak field strength in $x$ is about $4.18 \times 10^{8}$ V/m The beam waist radius is 200 μm. The corresponding pulse energy is about 16.9 μJ.

### S.5(vi) Parameters used to plot results in main text Figure 3.

In this section, we list the parameters used in our numerical results plotted in Figure 3 in the main text. Our numerical simulations for these cases do not account for space charge effects. We carried out simulations in both the plane wave and non-paraxial limits with $3.75 \times 10^{5}$ electrons.

We consider $\langle \mathrm{KE} \rangle = 5$ MeV electron bunches. During interaction, the electron bunches have radii of $\sigma_x = \sigma_y = 10$ μm and were spread over $\lambda_{gr}$ following a uniform random distribution. 4 different initial relative KE values were considered: $\sigma_{\mathrm{KE}}/\langle \mathrm{KE} \rangle = 0.02\%, 0.06\%, 0.10\%,$ and $0.14\%$. For simplicity, we assumed the momentum spread was isotropic in all directions, $\sigma_{\gamma\beta_x} = \sigma_{\gamma\beta_y} = \sigma_{\gamma\beta_z}$, the transverse momenta was vanishing, $\langle \gamma\beta_x \rangle = \langle \gamma\beta_y \rangle = 0$, and the mean longitudinal momentum was equal to the mean total momentum,$\langle \gamma\beta_z \rangle = \gamma_0\beta_0$. For this special case, we get $\sigma_\gamma/\beta_0 = \sigma_{\gamma\beta} = \sigma_{\gamma\beta_j}$, for $j \in \{x, y, z\}$ (see (S80)). For the above initial relative KE spread values, the corresponding $\sigma_{\gamma\beta_j} = \sigma_{\gamma\beta}$ values are: $\sigma_{\gamma\beta_j} = 1.9615 \times 10^{-3}$, $5.8848 \times 10^{-3}, 9.8075 \times 10^{-3}$, and $1.3731 \times$

$10^{-2}$. For Figures 3(a)-(c) in the main text, the results for the $\sigma_{\mathrm{KE}}/\langle\mathrm{KE}\rangle = 0.10\%$ have been omitted to keep the other results visible. Once again, the bunch was focused longitudinally and transversally down to the interaction region.

The laser pulses used in our non-paraxial simulations have beam waists of $w_0 = 300\ \mu\mathrm{m}$. The terahertz pulse has a (intensity) FWHM duration of 1 ps. The optical pulse has a (intensity) FWHM duration of 30 fs. The optical pulse energy was kept constant at 60 mJ. For our study, 4 different terahertz pulse energies are used: 0.52 μJ, 2.06 μJ, 4.65 μJ, and 8.26 μJ. These energies correspond to values of the product of peak field strengths, $E_{01}E_{02}$, of about (to within 1%) $0.5 \times 10^{19}\ \mathrm{V}^2/\mathrm{m}^2$, $1.0 \times 10^{19}\,\mathrm{V}^2/\mathrm{m}^2$, $1.5 \times 10^{19}\,\mathrm{V}^2/\mathrm{m}^2$, and $2.0 \times 10^{19}\,\mathrm{V}^2/\mathrm{m}^2$ in that order. The foci of both pulses were centered on the propagation axes, $x_{foc} = y_{foc} = 0$ m, and at $z_{foc} \approx 1.610413 \times 10^{-2}$ m. The initial optical and terahertz pulse peak positions relative to $z_{foc}$ were $z \approx -1.617374 \times 10^{-2}$ m and $z \approx 1.617374 \times 10^{-2}$ m respectively. The pulse peaks overlapped each other and the electron bunch at the same time. For Figures 3(d)-(f) in the main text, the results for $E_{01}E_{02} \approx 1.5 \times 10^{19}\ \mathrm{V}^2/\mathrm{m}^2$ were omitted to keep the other results visible.

The plane wave simulations were carried out using plane laser pulses with a Poisson pulse profile [3], making them valid in both the single-cycle and multi-cycle limits. The laser pulse parameters used were the same as those used for the non-paraxial pulse simulations.

## References


1. Murphy, N. C.; Wortis, R.; Atkinson, W. A. Generalized inverse participation ratio as a possible measure of localization for interacting systems. *Phys. Rev. B* **2011**, 83, 184206.
2. Hilbert, S. A.; Uiterwaal, C.; Barwick, B.; Batelaan, H.; Zewail, A. H. Temporal lenses for attosecond and femtosecond electron pulses. *PNAS* **2009**, 106, 10558.
3. Caron, C. F. R.; Potvliege, R. M. Free-space propagation of ultrashort pulses: space-time couplings in Gaussian pulse beams. *J. Mod. Opt.* **1999**, 46, 1881.
4. Kozak, M.; Eckstein, T.; Schonenberger, N.; Hommelhoff, P. Inelastic ponderomotive scattering of electrons at a high-intensity optical travelling wave in vacuum. *Nat. Phys.* **2017**, 13, 611.
5. Wong, L. J.; Kaminer, I.; Ilic, O.; Joannopoulos, J. D.; Soljacic, M. Towards graphene plasmon-based free-electron infrared to X-ray sources. *Nat. Photon.* **2015,** 10, 46**.**
6. Wong, L. J.; et al. Laser-induced linear-field particle acceleration in free space. *Sci. Rep.* **2017**, 7, 11159.

7. April, A. Ultrashort, strongly focused laser pulses in free space. In *Coherence and Ultrashort Pulse Laser Emission*: Duarte, F. J., Ed.; InTech: Rijeka, Croatia, 2010; p355.
8. Stratton, J. A. In *Electromagnetic theory*: Schiff, L. I., Ed.; McGraw-Hill: New York and London, 1941; p32.
9. Maxson, J.; Cesar, D.; Calmasini, G.; Ody, A.; Musumeci, P.; Alesini, D. Direct measurement of sub-10 fs relativistic electron beams with ultralow emittance. *Phys. Rev. Lett.* **2017**, 118, 154802.
